# Supplementary material for: Complex-variable MP2 theory applied to core-vacant states for the computation of Auger spectra
Source: arXiv:2505.02810 source file (2025-09-09)
Supplement: Supplementary file 1 [file Supporting_Information_Perturbative_correlation_treatment_for_Auger_spectra.pdf]

# Complex-variable MP2 theory applied to core-vacant states for the computation of Auger electron spectra

# Supporting Information

Florian Matz, Jan Philipp Drennhaus,
Anthuan Ferino-Pérez, and Thomas-C. Jagau

## 1 Explicit expressions for the EOMDIP-CCSD(2) $\sigma$ vectors

Using permutation operators $\mathcal{P}_{ij}$ and $\mathcal{P}_{ijk}$ defined as $\mathcal{P}_{ij}\, f(i,j) = f(i,j) - f(j,i)$ and $\mathcal{P}_{ijk}\, f(i,j,k) = f(i,j,k) + f(j,k,i) + f(k,i,j) - f(j,i,k) - f(i,k,j) - f(k,j,i)$, the $\sigma$ vectors used to solve the right-hand side EOMDIP-CCSD or EOMDIP-CCSD(2) eigenvalue equations can be written as

$$
\begin{aligned}
\sigma_{ij} =& \mathcal{P}_{ij}\Bigg[\sum_k r_{jk}\Big(f_i^k + \sum_a f_a^k t_i^a + \sum_{la}\langle kl||ia\rangle\, t_l^a + \sum_{lab}\langle kl||ab\rangle\left(t_i^a t_l^b + \frac{1}{2}t_{il}^{ab}\right)\Big) \\
&+ \frac{1}{2}\sum_{kla}\Big(r_{kjl}^a\left(\langle kl||ia\rangle - \sum_b \langle kl||ab\rangle\, t_i^b\right)\Big)\Bigg] + \sum_{ka} r_{ijk}^a\Big(f_a^k + \sum_{lb} t_l^b\,\langle kl||ab\rangle\Big) \\
&+\frac{1}{2}\sum_{kl} r_{kl}\Big(\langle kl||ij\rangle + \frac{1}{2}\sum_{ab}\langle kl||ab\rangle\left(t_{ij}^{ab} + \frac{1}{2}\mathcal{P}_{ij}\mathcal{P}_{ab}\, t_i^a t_j^b\right) + \sum_a \mathcal{P}_{ij}\langle kl||ia\rangle\, t_j^a\Big)
\end{aligned}
$$

and

$$
\begin{aligned}
\sigma_{ijk}^a =& \mathcal{P}_{kij}\Bigg[-\frac{1}{2}\sum_l r_{ijl}^a\Big(f_k^l + \sum_b f_b^l t_k^b + \sum_{mb}\langle lm||kb\rangle t_m^b + \sum_{mbc}\langle lm||bc\rangle\big(t_k^b t_m^c + \frac{1}{2}t_{km}^{bc}\big)\Big) \\
&+ \frac{1}{4}\sum_{lm} r_{lmk}^a\Big(\langle lm||ij\rangle + \frac{1}{2}\sum_{bc}\langle lm||bc\rangle\big(t_{ij}^{bc} + \frac{1}{2}\mathcal{P}_{ij}\mathcal{P}_{bc}t_i^b t_j^c\big) + \sum_b \mathcal{P}_{ij}\langle lm||ib\rangle t_j^b\Big) \\
&- \frac{1}{4}\sum_b t_{ij}^{ab}\Big(\sum_{lm} r_{lm}\langle lm||kb\rangle + \sum_{lmc}\big(r_{lmk}^c\langle lm||cb\rangle - r_{lm}t_k^c\langle lm||bc\rangle\big)\Big)
\end{aligned}
$$

$$
\begin{aligned}
&- \frac{1}{2}\sum_{l} r_{kl}\Bigg(\langle la||ij\rangle + \frac{1}{2}\sum_{bc}\langle la||bc\rangle\big(t_{ij}^{bc} + \frac{1}{2}\mathcal{P}_{ij}\mathcal{P}_{bc}t_i^b t_j^c\big) \\
&\qquad - \sum_{m} t_m^a\langle lm||ij\rangle - \sum_{mbc}\frac{1}{2}\langle lm||bc\rangle t_m^a\big(t_{ij}^{bc} + \frac{1}{2}\mathcal{P}_{ij}\mathcal{P}_{bc}t_i^b t_j^c\big) - \sum_{mb} t_m^a\mathcal{P}_{ij}\langle lm||ib\rangle t_j^b \\
&\qquad - \mathcal{P}_{ij}\Big(\sum_{b} t_i^b\langle la||jb\rangle - \sum_{mbc} t_i^b t_{jm}^{ac}\langle lm||bc\rangle + \sum_{mb} t_{im}^{ab}\langle lm||jb\rangle\Big) \\
&\qquad + \sum_{mbc} t_m^b t_{ij}^{ac}\langle lm||bc\rangle - \sum_{b} t_{ij}^{ab} f_b^l\Bigg)\Bigg] \\
&- \frac{1}{2}\mathcal{P}_{ijk}\sum_{lb}\Bigg[r_{ljk}^b\Bigg(\langle la||ib\rangle - \sum_{c} t_i^c\langle la||bc\rangle - \sum_{mc}\big(t_{im}^{ac} - t_i^c t_m^a\big)\langle lm||bc\rangle - \sum_{m} t_m^a\langle lm||ib\rangle\Bigg)\Bigg] \\
&+ \sum_{b}\Bigg[r_{ijk}^b\Bigg(f_b^a - \sum_{l} f_b^l t_l^a - \sum_{lmc} t_l^a t_m^c\langle lm||bc\rangle\Bigg)\Bigg]
\end{aligned}
$$

## 2 Computational Details

Table S1: Exponents of complex basis functions by atom type and angular momentum. In calculations with two complex-scaled shells we used the first two exponents (from top to bottom) per angular momentum. In calculations with four shells we used the first four, in calculations with five shells the first five and so on.

| Atom | s | p | d |
|---|---|---|---|
| H[a] | 0.398893 | 1.605600 | 2.184213 |
| | 0.129217 | 0.520551 | 0.386118 |
| | 0.258435 | 1.041103 | 0.772236 |
| | 0.064609 | 0.260276 | 0.193059 |
| H[b] | 0.330271317 | 1.329389259 | 1.808464179 |
| | 0.1069882 | 0.431001171 | 0.319694337 |
| | 0.2139764 | 0.862002265 | 0.639388599 |
| | 0.0534941 | 0.215500547 | 0.159847169 |
| | 0.02674705 | 0.107750274 | 0.079923584 |
| | 0.013373525 | 0.053875137 | 0.039961792 |
| | 0.006686762 | 0.026937568 | 0.019980896 |
| | 0.003343381 | 0.013468784 | 0.009990448 |
| | 0.0016716905 | 0.006734392 | 0.004995224 |
| | 0.00083584525 | 0.003367196 | 0.002497612 |
| C | 1.5775008 | 6.349666 | 8.637909 |
| | 0.5110162 | 2.0586245 | 1.526981 |

| Atom | s | p | d |
|---|---|---|---|
| N | 2.1804898 | 8.7767831 | 11.9396915 |
| | 0.7063487 | 2.8455199 | 2.1106592 |
| O | 2.775914 | 11.17345 | 15.200051 |
| | 0.899231 | 3.622543 | 2.687015 |
| | 1.798461 | 7.245086 | 5.374029 |
| | 0.449615 | 1.811272 | 1.343507 |
| Si | 1.651131563 | 6.646040548 | 9.041089 |
| | 0.534868106 | 2.154712201 | 1.59825387 |
| | 0.939754017 | 3.784217840 | 3.784218 |
| | 0.267434053 | 1.0773561005 | 0.799126935 |
| | 0.1337170265 | 0.53867805025 | 0.3995634675 |
| | 0.06685851325 | 0.269339025125 | 0.19978173375 |
| | 0.033429256625 | 0.1346695125625 | 0.099890866875 |
| | 0.0167146283125 | 0.06733475628125 | 0.0499454334375 |
| P | 2.027511835 | 8.161024942 | 11.10203 |
| | 0.656792856 | 2.645885154 | 1.962580518 |
| | 1.153973695 | 4.646841372 | 4.667829023 |
| | 0.328396428 | 1.322942577 | 0.981290259 |
| | 0.164198214 | 0.6614712885 | 0.4906451295 |
| | 0.082099107 | 0.33073564425 | 0.24532256475 |
| | 0.0410495535 | 0.165367822125 | 0.122661282375 |
| | 0.02052477675 | 0.0826839110625 | 0.0613306411875 |
| S | 2.381349933 | 9.585273863 | 13.03954 |
| | 0.771415287 | 3.107640767 | 2.305086907 |
| | 1.542830574 | 6.215280984 | 4.610173265 |
| | 0.385707644 | 1.553820109 | 1.152543454 |
| | 0.192853822 | 0.776910054 | 0.576271727 |
| | 0.096426911 | 0.388455027 | 0.288135863 |
| | 0.048213455 | 0.194227514 | 0.144067932 |
| | 0.024106728 | 0.097113757 | 0.072033966 |
| | 0.012053364 | 0.0485568785 | 0.036016983 |
| | 0.006026682 | 0.02427843925 | 0.0180084915 |

[a] with cc-pCVTZ (5sp) basis
[b] with aug-cc-pCVTZ (5sp) basis

Table S2: Structural parameters.

| Atom X | Distance $d_{XH}$/Å | Angle $A_{HXH}$/° |
|---|---|---|
| O | 0.961 92 | 104.805 37 |
| N | 1.015 90 | 106.267 46 |
| C | 1.090 48 | 109.471 22 |
| S | 1.333 76 | 92.205 47 |
| P | 1.420 97 | 93.303 09 |
| Si | 1.473 40 | 109.471 22 |

Table S3: Optimal complex-scaling angles for different molecules, states, methods, and basis sets in degree.

| Molecule | Complex-scaled shells[a] | K-shell ionization | | L-shell ionization | |
|---|---|---|---|---|---|
| | | CCSD | MP2 | EOM-CCSD | MP2 |
| $CH_4$ | 2(spd) | 13 | 12 | – | – |
| $NH_3$ | 2(spd) | 16 | 15 | – | – |
| $H_2O$ | 2(spd) | 16 | 17 | – | – |
| $H_2O$ | 4(spd) | – | 16 | – | – |
| $SiH_4$ | 2(spd) | 25 | 26 | – | 3 |
| $SiH_4$ | 4(spd) | – | – | – | 7 |
| $SiH_4$ | 5(spd) | – | – | – | 13 |
| $SiH_4$ | 6(spd) | – | – | 20 | 10 |
| $PH_3$ | 2(spd) | 28 | 36 | – | 7 |
| $PH_3$ | 4(spd) | – | – | – | 12 |
| $PH_3$ | 5(spd) | – | – | – | 10 |
| $PH_3$ | 6(spd) | – | – | 24 | 15 |
| $H_2S$ | 2(spd) | 30 | 40 | – | 13 |
| $H_2S$ | 4(spd) | 14 | 15 | 17 | 21 |
| $H_2S$ | 5(spd) | – | – | – | 12 |
| $H_2S$ | 6(spd) | – | – | 27 | 28 |
| $H_2S$ | 8(spd) | – | – | 14 | 7 |
| $H_2S$ | 10(spd) | – | – | – | 5 |

[a] The unscaled basis set is cc-pCVTZ(5sp) or aug-cc-pCVTZ(5sp) in all calculations. See main text for details.

## 3 Extrapolation of double ionization energies

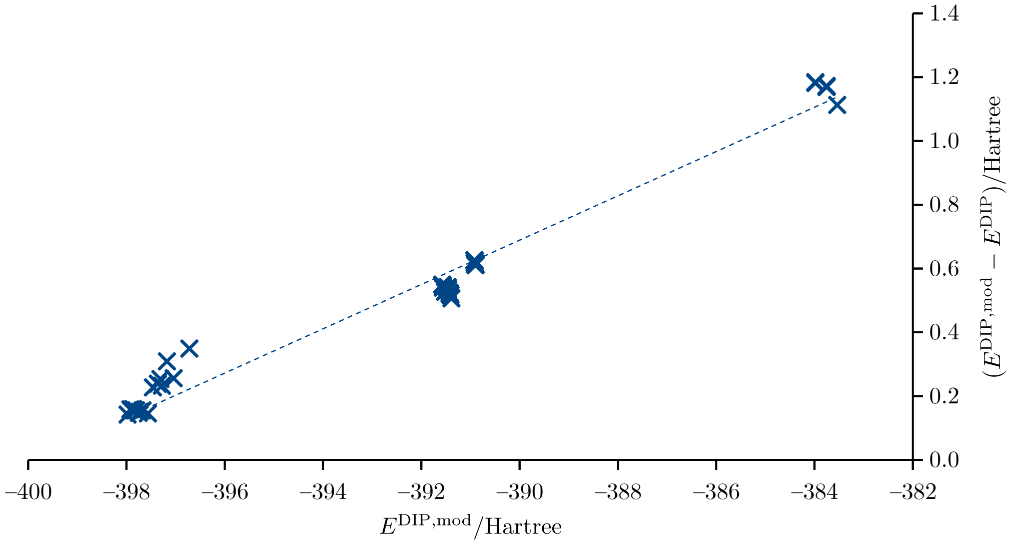


Figure S1: Energy difference between EOMDIP-CCSD energies for hydrogen sulfide computed with ($E^{\mathrm{DIP}}$) and without ($E^{\mathrm{DIP,mod}}$) $3h1p$ excitations as a function of $E^{\mathrm{DIP,mod}}$.

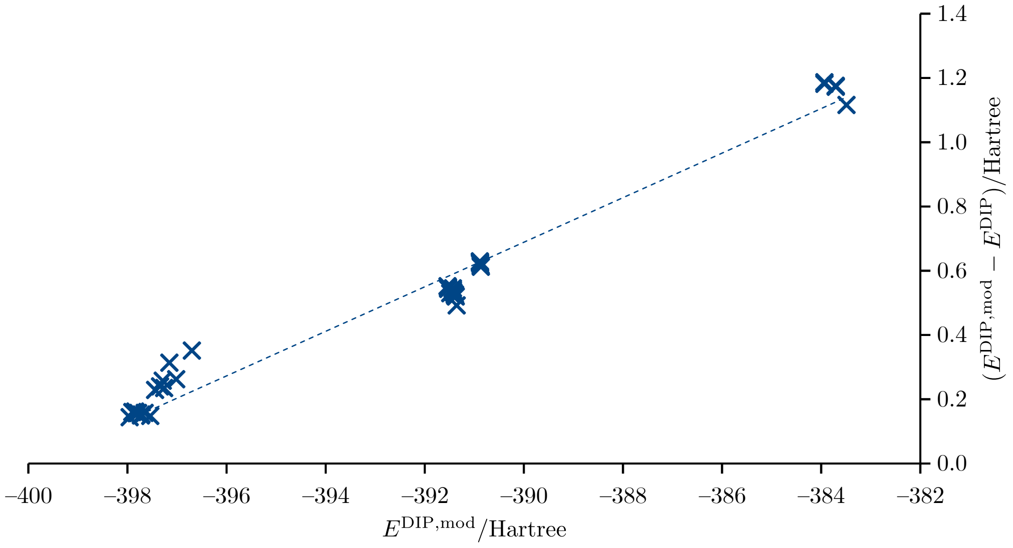


Figure S2: Energy difference between EOMDIP-CCSD(2) energies for hydrogen sulfide computed with ($E^{\mathrm{DIP}}$) and without ($E^{\mathrm{DIP,mod}}$) $3h1p$ excitations as a function of $E^{\mathrm{DIP,mod}}$.

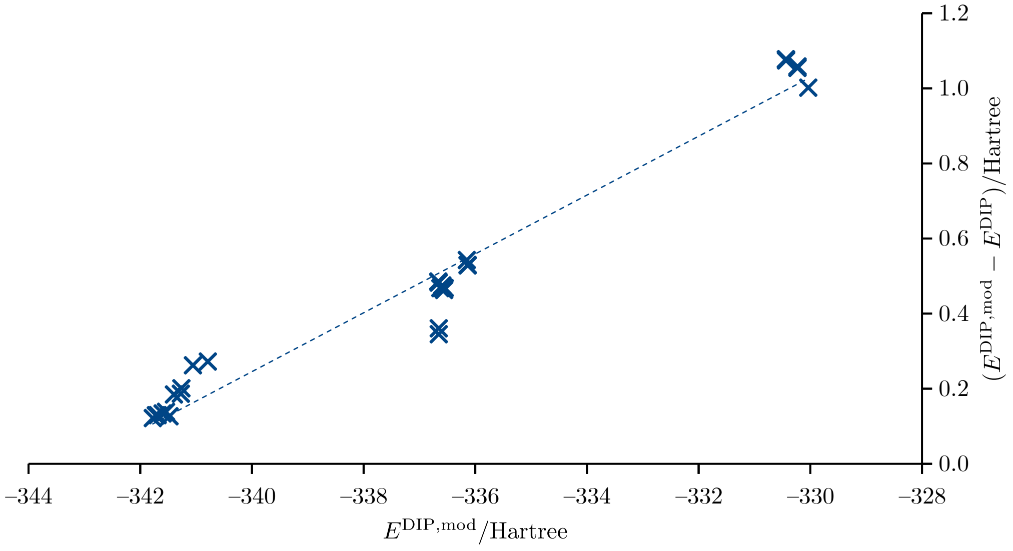


Figure S3: Energy difference between EOMDIP-CCSD energies for phosphine computed with ($E^{\mathrm{DIP}}$) and without ($E^{\mathrm{DIP,mod}}$) $3h1p$ excitations as a function of $E^{\mathrm{DIP,mod}}$.

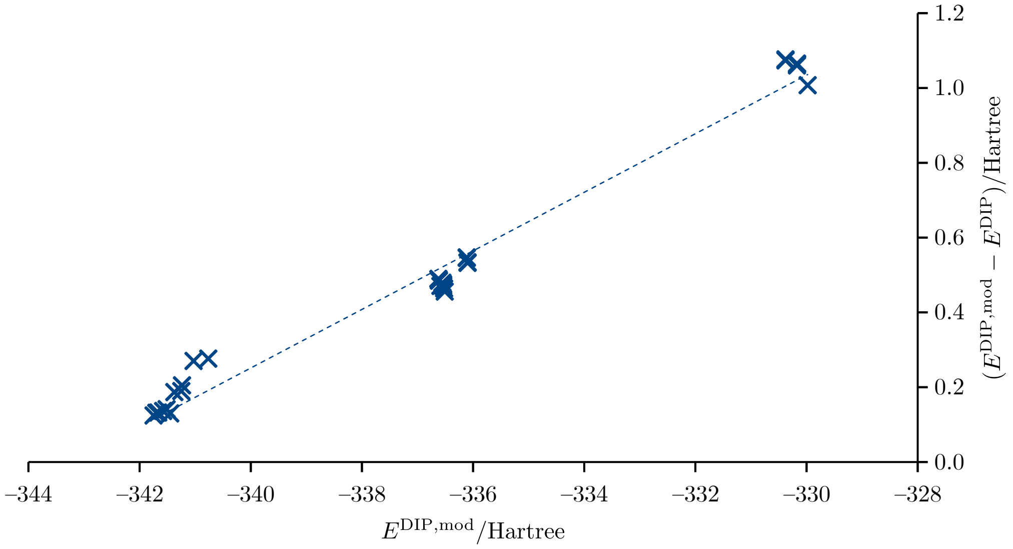


Figure S4: Energy difference between EOMDIP-CCSD(2) energies for phosphine computed with ($E^{\mathrm{DIP}}$) and without ($E^{\mathrm{DIP,mod}}$) $3h1p$ excitations as a function of $E^{\mathrm{DIP,mod}}$.

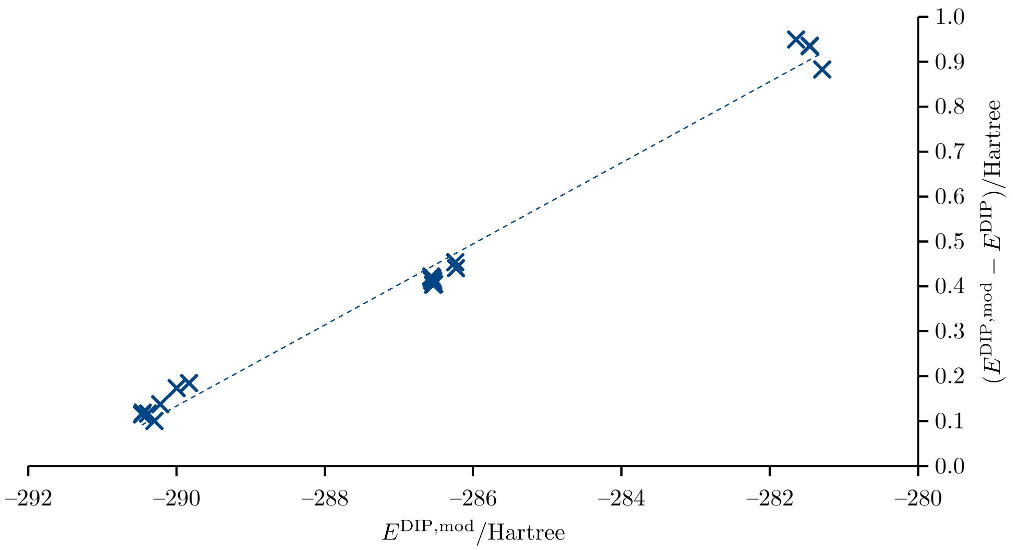


Figure S5: Energy difference between EOMDIP-CCSD energies for silane computed with ($E^{\mathrm{DIP}}$) and without ($E^{\mathrm{DIP,mod}}$) $3h1p$ excitations as a function of $E^{\mathrm{DIP,mod}}$.

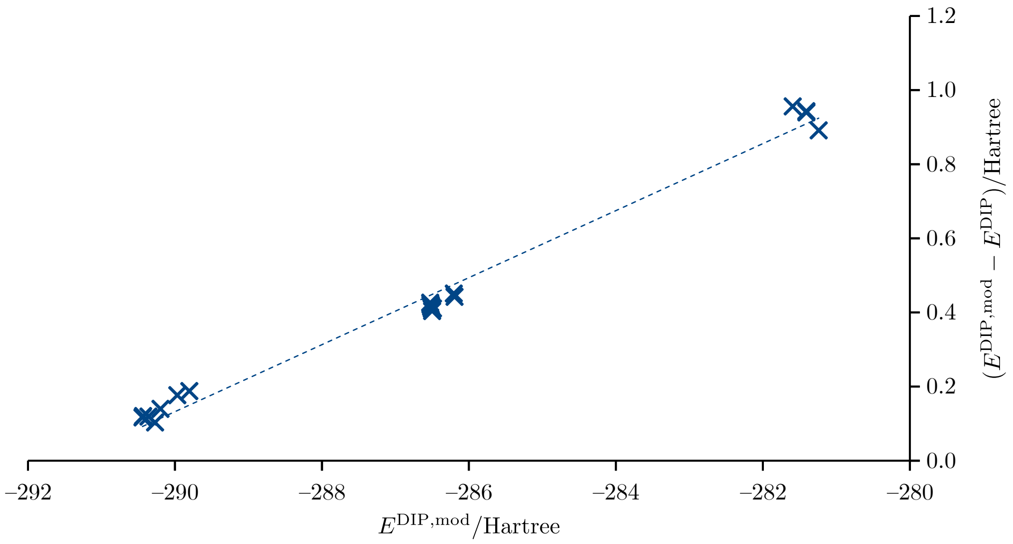


Figure S6: Energy difference between EOMDIP-CCSD(2) energies for silane computed with ($E^{\mathrm{DIP}}$) and without ($E^{\mathrm{DIP,mod}}$) $3h1p$ excitations as a function of $E^{\mathrm{DIP,mod}}$.

## 4 Partial decay widths

Table S4: Branching ratios for the Auger decay of the K-edge hole in hydrogen sulfide.

| Branch | $\sum \Gamma_{ij}$/meV | | | | $\sum \Gamma_{ij}/\Gamma$/% | | | | same width |
|---|---|---|---|---|---|---|---|---|---|
| #complex | CCSD | | MP2 | | CCSD | | MP2 | | for every |
| scaled shells: | 2 | 4 | 2 | 4 | 2 | 4 | 2 | 4 | channel |
| $L_1L_1$ | 24.6 | 22.3 | 25.8 | 27.8 | 5.5 | 4.9 | 5.8 | 5.6 | 1.6 |
| $L_1L_{2,3}$ | 125.4 | 122.1 | 127.8 | 126.0 | 28.1 | 27.0 | 28.5 | 25.5 | 9.4 |
| $L_1M_1$ | 4.4 | 2.9 | 5.0 | 3.1 | 1.0 | 0.6 | 1.1 | 0.6 | 3.1 |
| $L_1M_{2,3}$ | 7.6 | 7.7 | 7.6 | 7.5 | 1.7 | 1.7 | 1.7 | 1.5 | 9.4 |
| $L_{2,3}L_{2,3}$ | 249.6 | 258.2 | 247.2 | 290.4 | 55.9 | 57.1 | 55.2 | 58.7 | 14.1 |
| $L_{2,3}M_1$ | 8.2 | 8.5 | 8.2 | 8.6 | 1.8 | 1.9 | 1.8 | 1.7 | 9.4 |
| $L_{2,3}M_{2,3}$ | 25.6 | 28.8 | 24.8 | 30.1 | 5.7 | 6.4 | 5.6 | 6.1 | 28.1 |
| $M_1M_1$ | 0.2 | 0.1 | 0.2 | 0.1 | 0.1 | 0.0 | 0.1 | 0.0 | 1.6 |
| $M_1M_{2,3}$ | 0.4 | 0.5 | 0.6 | 0.5 | 0.1 | 0.1 | 0.1 | 0.1 | 9.4 |
| $M_{2,3}M_{2,3}$ | 0.6 | 0.8 | 0.6 | 0.8 | 0.1 | 0.2 | 0.1 | 0.2 | 14.1 |
| LL | 399.6 | 402.5 | 400.8 | 444.1 | 89.5 | 89.1 | 89.5 | 89.7 | 25 |
| LM | 45.8 | 47.9 | 45.6 | 49.3 | 10.2 | 10.6 | 10.2 | 10.4 | 50 |
| MM | 1.2 | 1.4 | 1.4 | 1.4 | 0.3 | 0.3 | 0.3 | 0.3 | 25 |

Table S5: Partial Auger decay widths in meV for the $1a_1^{-1}$ hole of methane, computed with two complex scaled shells per angular momentum (+2(spd)).

| Decay channel | CCSD | MP2 |
|---|---|---|
| $^1A_1$ ($2a_12a_1$) | 11.4 | 14.9 |
| $^1T_2$ ($2a_11t_2$) | 19.1 | 29.7 |
| $^3T_2$ ($2a_11t_2$) | 5.8 | 7.6 |
| $^1A_1$ ($1t_21t_2$) | 2.6 | 4.6 |
| $^1T_2$ ($1t_21t_2$) | 38.7 | 34.0 |
| $^1E$ ($1t_21t_2$) | 19.8 | 34.5 |
| $^3T_1$ ($1t_21t_2$) | 0.0 | 0.0 |
| Sum | 97.4 | 125.4 |

Table S6: Partial Auger decay widths in meV for the $1a_1^{-1}$ hole of ammonia, computed with two complex scaled shells per angular momentum (+2(spd)).

| Decay channel | CCSD | MP2 |
|---|---|---|
| $^1A_1$ ($2a_12a_1$) | 14.5 | 13.0 |
| $^1E$ ($2a_11e$) | 15.8 | 20.7 |
| $^3E$ ($2a_11e$) | 4.0 | 4.3 |
| $^1A_1$ ($2a_13a_1$) | 10.7 | 10.7 |
| $^3A_1$ ($2a_13a_1$) | 2.2 | 2.2 |
| $^1A_1$ (1e1e) | 6.4 | 8.6 |
| $^1E$ (1e1e) | 24.2 | 35.5 |
| $^3A_2$ (1e1e) | 0.0 | 0.0 |
| $^1E$ ($3a_11e$) | 28.4 | 46.6 |
| $^3E$ ($3a_11e$) | 0.3 | 0.3 |
| $^1A_1$ ($3a_13a_1$) | 13.5 | 20.8 |
| Sum | 119.9 | 162.7 |

Table S7: Partial Auger decay widths in meV for the $1a_1^{-1}$ hole of hydrogen sulfide, computed with two complex scaled shells per angular momentum (+2(spd)).

| Decay channel | CCSD | MP2 |
|---|---|---|
| $^3A_1$ ($2a_13a_1$) | 3.2 | 3.4 |
| $^3A_1$ ($2a_14a_1$) | 0.0 | 0.0 |
| $^3A_1$ ($2a_15a_1$) | 0.2 | 0.2 |
| $^1A_1$ ($2a_12a_1$) | 12.3 | 12.9 |
| $^1A_1$ ($2a_13a_1$) | 17.7 | 17.9 |
| $^1A_1$ ($2a_14a_1$) | 2.2 | 2.5 |
| $^1A_1$ ($2a_15a_1$) | 1.2 | 1.2 |
| $^3A_1$ ($3a_14a_1$) | 0.2 | 0.2 |
| $^3A_1$ ($3a_15a_1$) | 0.0 | 0.0 |
| $^1A_1$ ($3a_13a_1$) | 17.8 | 18.1 |
| $^1A_1$ ($3a_14a_1$) | 1.2 | 1.2 |
| $^1A_1$ ($3a_15a_1$) | 1.8 | 1.9 |
| $^3A_1$ ($4a_15a_1$) | 0.0 | 0.0 |
| $^1A_1$ ($4a_14a_1$) | 0.1 | 0.1 |
| $^1A_1$ ($4a_15a_1$) | 0.1 | 0.1 |
| $^1A_1$ ($5a_15a_1$) | 0.0 | 0.0 |
| $^3A_1$ ($1b_22b_2$) | 0.1 | 0.0 |
| $^1A_1$ ($1b_21b_2$) | 17.8 | 18.1 |
| $^1A_1$ ($2b_22b_2$) | 0.0 | 0.0 |
| $^3A_1$ ($1b_12b_1$) | 0.0 | 0.0 |

| Decay channel | CCSD | MP2 |
|---|---|---|
| $^1A_1$ ($1b_1 1b_1$) | 18.3 | 18.9 |
| $^1A_1$ ($1b_1 2b_1$) | 2.3 | 2.4 |
| $^1A_1$ ($2b_1 2b_1$) | 0.1 | 0.1 |
| $^1A_1$ ($1b_2 2b_2$) | 1.5 | 1.5 |
| $^3A_2$ ($1b_1 1b_2$) | 0.0 | 0.0 |
| $^3A_2$ ($1b_1 2b_2$) | 0.0 | 0.0 |
| $^1A_2$ ($1b_1 2b_2$) | 1.4 | 1.3 |
| $^3A_2$ ($2b_1 1b_2$) | 0.0 | 0.0 |
| $^1A_2$ ($2b_1 1b_2$) | 0.9 | 0.9 |
| $^3A_2$ ($2b_1 2b_2$) | 0.0 | 0.0 |
| $^1A_2$ ($2b_1 2b_2$) | 0.0 | 0.0 |
| $^1A_2$ ($1b_1 1b_2$) | 23.5 | 22.6 |
| $^3B_1$ ($2a_1 1b_1$) | 3.2 | 3.4 |
| $^3B_1$ ($2a_1 2b_1$) | 0.2 | 0.2 |
| $^1B_1$ ($2a_1 1b_1$) | 17.7 | 18.0 |
| $^1B_1$ ($2a_1 2b_1$) | 1.2 | 1.2 |
| $^3B_1$ ($3a_1 1b_1$) | 0.0 | 0.0 |
| $^3B_1$ ($3a_1 2b_1$) | 0.0 | 0.0 |
| $^1B_1$ ($3a_1 1b_1$) | 23.5 | 22.7 |
| $^1B_1$ ($3a_1 2b_1$) | 1.4 | 1.3 |
| $^3B_1$ ($4a_1 1b_1$) | 0.2 | 0.2 |
| $^3B_1$ ($4a_1 2b_1$) | 0.0 | 0.0 |
| $^1B_1$ ($4a_1 1b_1$) | 1.2 | 1.2 |
| $^1B_1$ ($4a_1 2b_1$) | 0.1 | 0.1 |
| $^3B_1$ ($5a_1 1b_1$) | 0.0 | 0.0 |
| $^3B_1$ ($5a_1 2b_1$) | 0.0 | 0.0 |
| $^1B_1$ ($5a_1 1b_1$) | 1.2 | 1.1 |
| $^1B_1$ ($5a_1 2b_1$) | 0.1 | 0.1 |
| $^3B_2$ ($2a_1 1b_2$) | 3.2 | 3.4 |
| $^3B_2$ ($2a_1 2b_2$) | 0.2 | 0.1 |
| $^1B_2$ ($2a_1 1b_2$) | 17.6 | 17.9 |
| $^1B_2$ ($2a_1 2b_2$) | 0.8 | 0.8 |
| $^3B_2$ ($3a_1 1b_2$) | 0.0 | 0.0 |
| $^3B_2$ ($3a_1 2b_2$) | 0.0 | 0.0 |
| $^1B_2$ ($3a_1 1b_2$) | 23.9 | 23.1 |
| $^1B_2$ ($3a_1 2b_2$) | 0.9 | 0.9 |
| $^3B_2$ ($4a_1 1b_2$) | 0.2 | 0.2 |
| $^3B_2$ ($4a_1 2b_2$) | 0.0 | 0.0 |
| $^1B_2$ ($4a_1 1b_2$) | 1.2 | 1.2 |
| $^1B_2$ ($4a_1 2b_2$) | 0.1 | 0.1 |
| $^3B_2$ ($5a_1 1b_2$) | 0.0 | 0.0 |
| $^3B_2$ ($5a_1 2b_2$) | 0.0 | 0.0 |

| Decay channel | CCSD | MP2 |
|---|---|---|
| $^1B_2$ ($5a_1 1b_2$) | 1.2 | 1.1 |
| $^1B_2$ ($5a_1 2b_2$) | 0.0 | 0.0 |

Table S8: Partial Auger decay widths in meV for the $1a_1^{-1}$ hole of phosphine, computed with two complex scaled shells per angular momentum (+2(spd)).

| Decay channel | CCSD | MP2 |
|---|---|---|
| $^1A_1$ ($2a_1 2a_1$) | 12.5 | 11.7 |
| $^1A_1$ ($2a_1 3a_1$) | 17.4 | 16.8 |
| $^1E$ ($2a_1 1e$) | 34.8 | 33.6 |
| $^1A_1$ ($2a_1 4a_1$) | 2.1 | 1.8 |
| $^1A_1$ ($2a_1 5a_1$) | 0.6 | 0.6 |
| $^1E$ ($2a_1 2e$) | 1.8 | 1.7 |
| $^1A_1$ ($3a_1 3a_1$) | 18.3 | 17.2 |
| $^1E$ ($3a_1 1e$) | 46.4 | 45.3 |
| $^1A_1$ ($3a_1 4a_1$) | 1.0 | 0.9 |
| $^1A_1$ ($3a_1 5a_1$) | 1.2 | 1.2 |
| $^1E$ ($3a_1 2e$) | 1.8 | 1.8 |
| $^1A_1$ (1e1e) | 13.4 | 11.6 |
| $^1E$ ($4a_1 1e$) | 2.0 | 1.9 |
| $^1E$ ($5a_1 1e$) | 1.4 | 1.5 |
| $^1A_1$+$^1A_2$+$^1E$ (1e2e) | 4.8 | 4.7 |
| $^1E$ (1e1e) | 46.6 | 45.5 |
| $^1A_1$ ($4a_1 4a_1$) | 0.1 | 0.1 |
| $^1A_1$ ($4a_1 5a_1$) | 0.0 | 0.0 |
| $^1E$ ($4a_1 2e$) | 0.1 | 0.1 |
| $^1A_1$ ($5a_1 5a_1$) | 0.0 | 0.0 |
| $^1E$ ($5a_1 2e$) | 0.1 | 0.1 |
| $^1A_1$ (2e2e) | 0.0 | 0.0 |
| $^1E$ (2e2e) | 0.1 | 0.1 |
| $^3A_1$ ($2a_1 3a_1$) | 3.3 | 3.1 |
| $^3E$ ($2a_1 1e$) | 6.7 | 6.3 |
| $^3A_1$ ($2a_1 4a_1$) | 0.0 | 0.0 |
| $^3A_1$ ($2a_1 5a_1$) | 0.1 | 0.1 |
| $^3E$ ($2a_1 2e$) | 0.3 | 0.3 |
| $^3E$ ($3a_1 1e$) | 0.0 | 0.0 |
| $^3A_1$ ($3a_1 4a_1$) | 0.1 | 0.1 |
| $^3A_1$ ($3a_1 5a_1$) | 0.0 | 0.0 |
| $^3E$ ($3a_1 2e$) | 0.0 | 0.0 |
| $^3E$ ($4a_1 1e$) | 0.3 | 0.3 |

| Decay channel | CCSD | MP2 |
|---|---|---|
| $^3$E (5a$_1$1e) | 0.0 | 0.0 |
| $^3$A$_1$+$^3$A$_2$+$^3$E (1e2e) | 0.1 | 0.1 |
| $^3$A$_2$ (1e1e) | 0.0 | 0.0 |
| $^3$A$_1$ (4a$_1$5a$_1$) | 0.0 | 0.0 |
| $^3$E (4a$_1$2e) | 0.0 | 0.0 |
| $^3$E (5a$_1$2e) | 0.0 | 0.0 |
| $^3$A$_2$ (2e2e) | 0.0 | 0.0 |

Table S9: Partial Auger decay widths in meV for the $1a_1^{-1}$ hole of silane, computed with two complex scaled shells per angular momentum (+2(spd)).

| Decay channel | CCSD | MP2 |
|---|---|---|
| $^1$A$_1$ (2a$_1$2a$_1$) | 9.9 | 11.4 |
| $^1$A$_1$ (2a$_1$3a$_1$) | 1.4 | 1.7 |
| $^1$T$_2$ (2a$_1$1t$_2$) | 50.1 | 46.8 |
| $^1$T$_2$ (2a$_1$2t$_2$) | 1.5 | 1.4 |
| $^1$A$_1$ (3a$_1$3a$_1$) | 0.1 | 0.1 |
| $^1$T$_2$ (3a$_1$1t$_2$) | 2.3 | 2.2 |
| $^1$T$_2$ (3a$_1$2t$_2$) | 0.1 | 0.1 |
| $^1$A$_1$+$^1$E (1t$_2$1t$_2$) | 56.1 | 48.4 |
| $^1$A$_1$+$^1$E (1t$_2$2t$_2$) | 3.1 | 2.8 |
| $^1$T$_1$ (1t$_2$1t$_2$) | 75.3 | 65.0 |
| $^1$T$_1$+$^1$T$_2$ (1t$_2$2t$_2$) | 3.9 | 3.5 |
| $^1$A$_1$+$^1$E (2t$_2$2t$_2$) | 0.0 | 0.0 |
| $^1$T$_1$ (2t$_2$2t$_2$) | 0.0 | 0.0 |
| $^3$A$_1$ (2a$_1$3a$_1$) | 0.0 | 0.0 |
| $^3$T$_2$ (2a$_1$1t$_2$) | 9.9 | 8.9 |
| $^3$T$_2$ (2a$_1$2t$_2$) | 0.3 | 0.3 |
| $^3$T$_2$ (3a$_1$1t$_2$) | 0.4 | 0.3 |
| $^3$T$_2$ (3a$_1$2t$_2$) | 0.0 | 0.0 |
| $^3$A$_1$+$^3$T$_1$ (1t$_2$2t$_2$) | 0.0 | 0.0 |
| $^3$T$_2$ (1t$_2$1t$_2$) | 0.0 | 0.0 |
| $^3$E (1t$_2$2t$_2$) | 0.0 | 0.0 |
| $^3$T$_2$ (2t$_2$2t$_2$) | 0.0 | 0.0 |

Table S10: Partial Auger decay widths in meV for the $2a_1^{-1}$ hole of hydrogen sulfide, computed with MP2/aug-cc-pCVTZ (5sp) and different numbers of complex-scaled functions.

| **Decay Channel** | 2(spd) | 4(spd) | 5(spd) | 6(spd) | 8(spd) | 10(spd) |
|---|---|---|---|---|---|---|
| $^3A_1$ ($3a_14a_1$) | 0.0 | 0.1 | 0.0 | 0.1 | 0.0 | 0.0 |
| $^3A_1$ ($3a_15a_1$) | 0.4 | 4.6 | 0.1 | –7.4 | 0.1 | 0.0 |
| $^3B_2$ ($3a_12b_2$) | 0.4 | 6.8 | –0.1 | –8.6 | 0.0 | 0.0 |
| $^3B_1$ ($3a_12b_1$) | 4.1 | 28.2 | 53.8 | 173.0 | 68.2 | 5.5 |
| $^1A_1$ ($3a_14a_1$) | 0.0 | 0.2 | 0.0 | –0.1 | 0.0 | 0.0 |
| $^1A_1$ ($3a_15a_1$) | 0.3 | 3.5 | 0.1 | –0.1 | 0.0 | 0.0 |
| $^1B_2$ ($3a_12b_2$) | 0.3 | 7.6 | –0.1 | –10.1 | 0.0 | 0.0 |
| $^1B_1$ ($3a_12b_1$) | 7.7 | 147.9 | 66.6 | 53.7 | 1.7 | 0.0 |
| $^3A_1$ ($4a_15a_1$) | 2.2 | 6.7 | 8.0 | 7.4 | 8.6 | 9.4 |
| $^3B_2$ ($4a_11b_2$) | 0.0 | 0.0 | 0.0 | 0.0 | 0.0 | 0.0 |
| $^3B_2$ ($4a_12b_2$) | 1.7 | 5.1 | 7.2 | 5.7 | 5.4 | 7.8 |
| $^3B_1$ ($4a_11b_1$) | 0.0 | 0.0 | 0.0 | –0.1 | 0.0 | 0.0 |
| $^3B_1$ ($4a_12b_1$) | 3.0 | 10.6 | 7.8 | 9.2 | 12.1 | 8.4 |
| $^1A_1$ ($4a_14a_1$) | 9.1 | 12.9 | 13.9 | 13.5 | 9.9 | 9.6 |
| $^1A_1$ ($4a_15a_1$) | 5.3 | 11.9 | 13.1 | 13.0 | 14.8 | 17.2 |
| $^1B_2$ ($4a_11b_2$) | 0.1 | 0.4 | 0.0 | –0.4 | 0.0 | 0.0 |
| $^1B_2$ ($4a_12b_2$) | 3.1 | 8.7 | 12.0 | 9.7 | 9.2 | 13.2 |
| $^1B_1$ ($4a_11b_1$) | 0.0 | 0.0 | 0.0 | 0.0 | 0.0 | 0.0 |
| $^1B_1$ ($4a_12b_1$) | 4.9 | 17.1 | 12.5 | 14.7 | 19.5 | 13.4 |
| $^3B_2$ ($5a_11b_2$) | 159.2 | 1451.3 | –4.5 | 255.3 | 2.1 | –0.4 |
| $^3B_2$ ($5a_12b_2$) | 0.2 | 0.7 | 0.7 | 0.6 | 0.8 | 0.8 |
| $^3B_1$ ($5a_11b_1$) | 0.3 | 2.4 | 0.4 | –2.1 | 0.0 | 0.0 |
| $^3B_1$ ($5a_12b_1$) | 0.5 | 1.2 | 0.7 | 1.0 | 1.2 | 1.4 |
| $^1A_1$ ($5a_15a_1$) | 1.7 | 2.8 | 2.3 | 2.6 | 3.3 | 2.3 |
| $^1B_2$ ($5a_11b_2$) | 18.3 | 212.5 | 0.1 | 24.5 | 0.2 | –0.1 |
| $^1B_2$ ($5a_12b_2$) | 0.3 | 1.4 | 1.4 | 1.1 | 1.5 | 1.6 |
| $^1B_1$ ($5a_11b_1$) | 0.2 | 2.7 | 0.2 | –2.8 | 0.0 | 0.0 |
| $^1B_1$ ($5a_12b_1$) | 0.9 | 2.1 | 1.2 | 1.7 | 2.0 | 2.4 |
| $^3A_1$ ($1b_22b_2$) | 0.2 | –1.5 | 0.0 | 4.5 | 0.0 | 0.0 |
| $^3A_2$ ($1b_22b_1$) | 6.4 | 40.3 | 60.5 | 647.6 | 1520.8 | 6.6 |
| $^1A_1$ ($1b_22b_2$) | 0.0 | –1.8 | 0.0 | 5.1 | 0.0 | 0.0 |
| $^1A_2$ ($1b_22b_1$) | 2.3 | 16.0 | 14.7 | 2.8 | 0.1 | 0.0 |
| $^3A_2$ ($2b_21b_1$) | 0.2 | 2.8 | 0.0 | –1.7 | 0.0 | 0.0 |
| $^3A_2$ ($2b_22b_1$) | 0.0 | 0.0 | 0.0 | 0.0 | 0.0 | 0.0 |
| $^1A_1$ ($2b_22b_2$) | 0.3 | 0.3 | 0.2 | 0.2 | 0.2 | 0.3 |
| $^1A_2$ ($2b_21b_1$) | 0.1 | 3.3 | 0.0 | –1.9 | 0.0 | 0.0 |
| $^1A_2$ ($2b_22b_1$) | 0.0 | 0.0 | 0.0 | 0.1 | 0.0 | 0.0 |

| **Decay Channel** | 2(spd) | 4(spd) | 5(spd) | 6(spd) | 8(spd) | 10(spd) |
|---|---|---|---|---|---|---|
| $^3A_1$ ($1b_12b_1$) | 166.3 | 1004.4 | 191.0 | 292.0 | 30.1 | 0.8 |
| $^1A_1$ ($1b_12b_1$) | 121.4 | 406.7 | 19060.3 | 2328.9 | 20.0 | 5.2 |
| $^1A_1$ ($2b_12b_1$) | 0.7 | 0.5 | 0.5 | 0.5 | 0.6 | 0.9 |

Table S11: Partial Auger decay widths in meV for the $2a_1^{-1}$ state of silane computed with the modified MP2 method using the aug-cc-pCVTZ (5sp) basis set with 5 complex-scaled sets of s-, p-, and d-shells.

| $L_{2,3}M$ channels | | MM channels | |
|---|---|---|---|
| Decay channel | Partial width | Decay channel | Partial width |
| $^1T_2$ ($3a_1^{-1}1t_2^{-1}$) | 415.9 | $^1T_2$ ($3a_1^{-1}2t_2^{-1}$) | 8.5 |
| $^1T_1$+$^1T_2$ ($1t_1^{-1}2t_1^{-1}$) | 137.4 | $^3T_2$ ($3a_1^{-1}2t_2^{-1}$) | 4.2 |
| $^3T_1$+$^3T_2$ ($1t_2^{-1}2t_2^{-1}$) | 103.8 | $^1A_1$ ($3a_1^{-2}$) | 3.5 |
| $^3A_1$+$^3E$ ($1t_2^{-1}1t_2^{-1}$) | 38.7 | $^1A_1$+$^1E$ ($2t_2^{-2}$) | 0.2 |
| $^1A_1$+$^1E$ ($1t_2^{-1}2t_2^{-1}$) | 34.9 | $^1T_1$ ($2t_2^{-2}$) | 0.1 |
| $^3T_2$ ($3a_1^{-1}1t_2^{-1}$) | 2.9 | $^3T_2$ ($2t_2^{-2}$) | 0.0 |
| Sum | 733.7 | Sum | 16.4 |

Table S12: Partial Auger decay widths in meV for the $2a_1^{-1}$ state of phosphine computed with the modified MP2 method, using the aug-cc-pCVTZ (5sp) basis set with 5 complex-scaled sets of s-, p-, and d-shells.

| $L_{2,3}M$ channels | | MM channels | |
|---|---|---|---|
| Decay channel | Partial width | Decay channel | Partial width |
| $^1E$ ($4a_1^{-1}1e^{-1}$) | 247.6 | $^1E$ ($4a_1^{-1}2e^{-1}$) | 7.8 |
| $^1A_1$+$^1A_2$+$^1E$ ($1e^{-1}2e^{-1}$) | 124.0 | $^1A_1$ ($4a_1^{-2}$) | 4.7 |
| $^1A_1$ ($3a_1^{-1}4a_1^{-1}$) | 90.8 | $^3E$ ($4a_1^{-1}2e^{-1}$) | 3.9 |
| $^3A_1$+$^3A_2$+$^3E$ ($1e^{-1}2e^{-1}$) | 77.7 | $^1A_1$ ($4a_1^{-1}5a_1^{-1}$) | 3.2 |
| $^1E$ ($3a_1^{-1}2e^{-1}$) | 73.4 | $^3A_1$ ($4a_1^{-1}5a_1^{-1}$) | 1.6 |
| $^1E$ ($5a_1^{-1}1e^{-1}$) | 57.0 | $^1A_1$ ($2e^{-2}$) | 1.2 |
| $^3E$ ($5a_1^{-1}1e^{-1}$) | 47.7 | $^1E$ ($2e^{-2}$) | 0.8 |
| $^3E$ ($3a_1^{-1}2e^{-1}$) | 46.7 | $^1E$ ($5a_1^{-1}2e^{-1}$) | 0.4 |
| $^1A_1$ ($3a_1^{-1}5a_1^{-1}$) | 21.7 | $^3E$ ($5a_1^{-1}2e^{-1}$) | 0.2 |
| $^3A_1$ ($3a_1^{-1}5a_1^{-1}$) | 21.2 | $^3A_2$ ($2e^{-2}$) | 0.2 |
| $^3E$ ($4a_1^{-1}1e^{-1}$) | 3.9 | $^1A_1$ ($5a_1^{-2}$) | 0.1 |
| $^3A_1$ ($3a_1^{-1}4a_1^{-1}$) | 2.3 | | |
| Sum | 814.1 | Sum | 24.1 |

Table S13: Partial Auger decay widths in meV for the $2a_1^{-1}$ state of hydrogen sulfide computed with the modified MP2 method in comparison to ACP-EOMIP-CCSD results, using the aug-cc-pCVTZ (5sp) basis set with 8 complex scaled sets of s-, p-, and d-shells.

| $L_{2,3}M$ channels | | | MM channels | | |
|---|---|---|---|---|---|
| Decay channel | ACP | MP2-mod | Decay channel | ACP | MP2-mod |
| $^1B_1$ $(4a_1^{-1}1b_1^{-1})$ | 244.3 | 281.7 | $^1B_1$ $(4a_1^{-1}2b_1^{-1})$ | 9.3 | 10.1 |
| $^1A_1$ $(3a_1^{-1}4a_1^{-1})$ | 236.4 | 288.1 | $^1A_1$ $(4a_1^{-2})$ | 7.5 | 17.3 |
| $^1B_2$ $(4a_1^{-1}1b_2^{-1})$ | 208.7 | 326.3 | $^1A_1$ $(4a_1^{-1}5a_1^{-1})$ | 7.2 | 10.7 |
| $^1A_1$ $(1b_1^{-1}2b_1^{-1})$ | 97.8 | 155.4 | $^1B_2$ $(4a_1^{-1}2b_2^{-1})$ | 5.9 | 8.6 |
| $^1A_1$ $(3a_1^{-1}5a_1^{-1})$ | 97.2 | 166.0 | $^3B_1$ $(4a_1^{-1}2b_1^{-1})$ | 3.8 | 5.5 |
| $^3A_1$ $(1b_1^{-1}2b_1^{-1})$ | 76.1 | 85.0 | $^3A_1$ $(4a_1^{-1}5a_1^{-1})$ | 3.2 | 5.1 |
| $^1A_1$ $(1b_2^{-1}2b_2^{-1})$ | 65.2 | 111.7 | $^1A_1$ $(5a_1^{-2})$ | 2.7 | 2.3 |
| $^3A_1$ $(1b_2^{-1}2b_2^{-1})$ | 59.8 | 76.4 | $^3B_2$ $(4a_1^{-1}2b_2^{-1})$ | 2.4 | 4.4 |
| $^3A_1$ $(3a_1^{-1}5a_1^{-1})$ | 57.3 | 79.0 | $^1B_1$ $(5a_1^{-1}2b_1^{-1})$ | 0.8 | 1.1 |
| $^1B_1$ $(5a_1^{-1}1b_1^{-1})$ | 43.0 | 73.1 | $^1B_2$ $(5a_1^{-1}2b_2^{-1})$ | 0.6 | 0.8 |
| $^3B_2$ $(3a_1^{-1}2b_2^{-1})$ | 34.1 | 41.6 | $^3B_1$ $(5a_1^{-1}2b_1^{-1})$ | 0.5 | 0.6 |
| $^1B_2$ $(5a_1^{-1}1b_2^{-1})$ | 33.6 | 64.9 | $^1A_1$ $(2b_1^{-2})$ | 0.4 | 0.6 |
| $^3A_2$ $(1b_2^{-1}2b_1^{-1})$ | 32.6 | 36.3 | $^3B_2$ $(5a_1^{-1}2b_2^{-1})$ | 0.3 | 0.4 |
| $^3B_1$ $(3a_1^{-1}2b_1^{-1})$ | 32.2 | 34.4 | $^1A_1$ $(2b_2^{-2})$ | 0.1 | 0.3 |
| $^3A_2$ $(2b_2^{-1}1b_1^{-1})$ | 30.6 | 41.7 | $^3A_2$ $(2b_2^{-1}2b_1^{-1})$ | 0.0 | 0.0 |
| $^3B_1$ $(5a_1^{-1}1b_1^{-1})$ | 26.7 | 35.3 | $^1A_2$ $(2b_2^{-1}2b_1^{-1})$ | −0.6 | 0.0 |
| $^3B_2$ $(5a_1^{-1}1b_2^{-1})$ | 22.9 | 35.0 | | | |
| $^1B_2$ $(3a_1^{-1}2b_2^{-1})$ | 9.2 | 39.4 | | | |
| $^1A_2$ $(2b_2^{-1}1b_1^{-1})$ | 8.8 | 39.2 | | | |
| $^1A_2$ $(1b_2^{-1}2b_1^{-1})$ | 8.3 | 33.0 | | | |
| $^1B_1$ $(3a_1^{-1}2b_1^{-1})$ | 6.3 | 31.3 | | | |
| $^3B_1$ $(4a_1^{-1}1b_1^{-1})$ | –5.3 | 3.6 | | | |
| $^3A_1$ $(3a_1^{-1}4a_1^{-1})$ | –13.7 | 5.9 | | | |
| $^3B_2$ $(4a_1^{-1}1b_2^{-1})$ | –15.6 | 5.4 | | | |
| Sum | 1396.5 | 2089.7 | Sum | 44.1 | 67.8 |

Table S14: Comparison of KLL partial decay widths of water and hydrogen sulfide computed with CCSD in the aug-cc-pCVTZ(5sp)+2(spd) basis. Relative intensities with respect to the largest partial width are shown as well.

| | $H_2O$ | | $H_2S$ | |
|---|---|---|---|---|
| Decay channel | $\Gamma_{ij}$/meV | $\Gamma_{ij}/\max(\Gamma_{ij})$ | $\Gamma_{ij}$/meV | $\Gamma_{ij}/\max(\Gamma_{ij})$ |
| $^1A_1$ ($2a_12a_1$) | 16.7 | 0.96 | 24.6 | 0.51 |
| $^1A_1$ ($2a_13a_1$) | 13.5 | 0.77 | 35.3 | 0.74 |
| $^1B_2$ ($2a_11b_2$) | 7.3 | 0.41 | 35.3 | 0.74 |
| $^1B_1$ ($2a_11b_1$) | 12.3 | 0.71 | 35.4 | 0.74 |
| $^1A_1$ ($3a_13a_1$) | 11.7 | 0.67 | 35.7 | 0.75 |
| $^1A_1$ ($1b_21b_2$) | 10.1 | 0.57 | 35.5 | 0.74 |
| $^1A_1$ ($1b_11b_1$) | 16.5 | 0.94 | 36.6 | 0.77 |
| $^1B_2$ ($3a_11b_2$) | 17.5 | 1.00 | 47.8 | 1.00 |
| $^1B_1$ ($3a_11b_1$) | 16.4 | 0.94 | 47.0 | 0.98 |
| $^1A_2$ ($1b_11b_2$) | 14.2 | 0.81 | 46.9 | 0.98 |
| $^3A_1$ ($2a_13a_1$) | 2.4 | 0.14 | 6.5 | 0.14 |
| $^3B_2$ ($2a_11b_2$) | 1.9 | 0.11 | 6.5 | 0.14 |
| $^3B_1$ ($2a_11b_1$) | 2.9 | 0.17 | 6.5 | 0.14 |
| $^3B_2$ ($3a_11b_2$) | 0.2 | 0.01 | 0.0 | 0.00 |
| $^3B_1$ ($3a_11b_1$) | 0.3 | 0.02 | 0.0 | 0.00 |
| $^3A_2$ ($1b_11b_2$) | 0.0 | 0.00 | 0.0 | 0.00 |

# 5 Energies of doubly ionized states

Table S15: EOMDIP-CCSD and EOMDIP-CCSD(2) total energies in Hartree for dicationic states of methane. The column "Weight" reports the square of the amplitude of the respective configuration divided by the square norm of $R_{ij}$. The energy of the neutral ground state is -40.49028/-40.46879 a.u. computed with CCSD and MP2, respectively.

| | | EOMDIP-CCSD | | | EOMDIP-CCSD(2) | | |
|---|---|---|---|---|---|---|---|
| Spin state | Configuration | Total energy | Weight | Partial width | Total energy | Weight | Partial width |
| S | $1b_1 1b_1$ | -39.04666 | 0.659 | 3.4 | -39.02977 | 0.647 | 4.4 |
| | $1b_2 1b_2$ | | 0.233 | | | 0.273 | |
| | $1b_3 1b_3$ | | 0.109 | | | 0.079 | |
| S | $1b_3 1b_3$ | -39.04666 | 0.560 | 3.4 | -39.02977 | 0.588 | 4.4 |
| | $1b_2 1b_2$ | | 0.432 | | | 0.392 | |
| | $1b_1 1b_1$ | | 0.008 | | | 0.020 | |
| S | $1b_3 1b_3$ | -38.93056 | 0.312 | 3.5 | -38.91034 | 0.312 | 4.6 |
| | $1b_2 1b_2$ | | 0.312 | | | 0.312 | |
| | $1b_1 1b_1$ | | 0.312 | | | 0.312 | |
| | 2a2a | | 0.063 | | | 0.064 | |
| S | 2a2a | -38.25133 | 0.930 | 4.5 | -38.23262 | 0.929 | 5.8 |
| | $1b_2 1b_2$ | | 0.023 | | | 0.024 | |
| | $1b_3 1b_3$ | | 0.023 | | | 0.024 | |
| | $1b_1 1b_1$ | | 0.023 | | | 0.024 | |
| S | $1b_2 1b_3$ | -38.99876 | 0.958 | 5.6 | -38.98013 | 0.956 | 5.0 |
| | $2a1b_1$ | | 0.042 | | | 0.044 | |
| S | $2a1b_1$ | -38.54354 | 0.962 | 2.7 | -38.52074 | 0.959 | 4.1 |
| | $1b_2 1b_3$ | | 0.038 | | | 0.041 | |
| S | $1b_1 1b_3$ | -38.99876 | 0.958 | 5.6 | -38.98013 | 0.956 | 5.0 |
| | $2a1b_2$ | | 0.042 | | | 0.044 | |
| S | $2a1b_2$ | -38.54354 | 0.962 | 2.7 | -38.52074 | 0.959 | 4.1 |
| | $1b_1 1b_3$ | | 0.038 | | | 0.041 | |
| S | $1b_1 1b_2$ | -38.99876 | 0.958 | 5.6 | -38.98013 | 0.956 | 5.0 |
| | $2a1b_3$ | | 0.042 | | | 0.044 | |
| S | $2a1b_3$ | -38.54354 | 0.962 | 2.7 | -38.52074 | 0.959 | 4.1 |
| | $1b_1 1b_2$ | | 0.038 | | | 0.041 | |
| T | $1b_2 1b_3$ | -39.07219 | 1.000 | 0.0 | -39.05541 | 1.000 | 0.0 |
| T | $2a1b_1$ | -38.74517 | 1.000 | 0.8 | -38.72490 | 1.000 | 1.1 |
| T | $1b_1 1b_3$ | -39.07219 | 1.000 | 0.0 | -39.05541 | 1.000 | 0.0 |
| T | $2a1b_2$ | -38.74517 | 1.000 | 0.8 | -38.72490 | 1.000 | 1.1 |
| T | $1b_1 1b_2$ | -39.07219 | 1.000 | 0.0 | -39.05541 | 1.000 | 0.0 |
| T | $2a1b_3$ | -38.74517 | 1.000 | 0.8 | -38.72490 | 1.000 | 1.1 |

Table S16: EOMDIP-CCSD and EOMDIP-CCSD(2) total energies in Hartree for dicationic states of ammonia. The column "Weight" reports the square of the amplitude of the respective configuration divided by the square norm of $R_{ij}$. The energy of the neutral ground state is -56.53140/-56.51861 computed with CCSD and MP2, respectively.

| | | EOMDIP-CCSD | | | EOMDIP-CCSD(2) | | |
|---|---|---|---|---|---|---|---|
| Spin state | Configuration | Total energy | Weight | Partial width | Total energy | Weight | Partial width |
| S | 4a'4a' | -55.19626 | 0.985 | 3.0 | -55.17821 | 0.984 | 4.6 |
| | 2a'2a' | | 0.004 | | | 0.004 | |
| | 1a"1a" | | 0.003 | | | 0.003 | |
| | 3a'3a' | | 0.003 | | | 0.003 | |
| | 2a'4a' | | 0.005 | | | 0.005 | |
| S | 3a'4a' | -55.04818 | 0.998 | 3.1 | -55.03361 | 0.998 | 5.2 |
| | 1a"1a" | | 0.001 | | | 0.001 | |
| | 3a'3a' | | 0.001 | | | 0.001 | |
| | 2a'3a' | | 0.001 | | | 0.001 | |
| S | 3a'3a' | -54.83827 | 0.493 | 2.1 | -54.82580 | 0.493 | 2.9 |
| | 1a"1a" | | 0.493 | | | 0.493 | |
| | 2a'3a' | | 0.012 | | | 0.013 | |
| | 3a'4a' | | 0.001 | | | 0.001 | |
| S | 1a"1a" | -54.77658 | 0.477 | 2.1 | -54.76275 | 0.477 | 3.0 |
| | 3a'3a' | | 0.477 | | | 0.477 | |
| | 2a'2a' | | 0.037 | | | 0.037 | |
| | 4a'4a' | | 0.006 | | | 0.006 | |
| | 2a'4a' | | 0.003 | | | 0.003 | |
| S | 2a'4a' | -54.49429 | 0.988 | 2.3 | -54.47889 | 0.989 | 2.3 |
| | 2a'2a' | | 0.004 | | | 0.004 | |
| | 4a'4a' | | 0.003 | | | 0.004 | |
| | 3a'3a' | | 0.002 | | | 0.002 | |
| | 1a"1a" | | 0.002 | | | 0.002 | |
| S | 2a'3a' | -54.25147 | 0.988 | 1.6 | -54.23860 | 0.987 | 2.0 |
| | 3a'3a' | | 0.006 | | | 0.006 | |
| | 1a"1a" | | 0.006 | | | 0.006 | |
| | 3a'4a' | | 0.001 | | | 0.001 | |
| S | 2a'2a' | -53.85315 | 0.951 | 2.7 | -53.84149 | 0.951 | 2.5 |
| | 3a'3a' | | 0.016 | | | 0.016 | |
| | 1a"1a" | | 0.016 | | | 0.016 | |
| | 2a'4a' | | 0.012 | | | 0.012 | |
| | 4a'4a' | | 0.005 | | | 0.006 | |
| S | 4a'1a" | -55.04818 | 0.998 | 3.1 | | 0.998 | 5.2 |

| | | EOMDIP-CCSD | | | EOMDIP-CCSD(2) | | |
|---|---|---|---|---|---|---|---|
| Spin | Transition | Total | Weight | Partial | Total | Weight | Partial |
| | 3a'1a" | | 0.001 | | -55.03361 | 0.001 | |
| | 2a'1a" | | 0.001 | | | 0.001 | |
| S | 3a'1a" | -54.83827 | 0.987 | 2.7 | | 0.986 | 3.9 |
| | 2a'1a" | | 0.012 | | -54.82580 | 0.013 | |
| | 4a'1a" | | 0.001 | | | 0.001 | |
| S | 2a'1a" | -54.25147 | 0.988 | 1.6 | | 0.987 | 2.0 |
| | 3a'1a" | | 0.011 | | -54.23860 | 0.012 | |
| | 4a'1a" | | 0.001 | | | 0.001 | |
| T | 3a'4a' | -55.10396 | 0.999 | 0.0 | | 0.999 | 0.0 |
| | 2a'3a' | | 0.001 | | -55.08964 | 0.001 | |
| T | 2a'4a' | -54.67446 | 1.000 | 0.5 | | 1.000 | 0.5 |
| T | 2a'3a' | -54.47494 | 0.998 | 0.4 | -54.65999 | 0.998 | 0.5 |
| | 3a'4a' | | 0.002 | | -54.46314 | 0.002 | |
| T | 4a'1a" | -55.10396 | 0.999 | 0.0 | | 0.999 | 0.0 |
| | 2a'1a" | | 0.001 | | -55.08964 | 0.001 | |
| T | 3a'1a" | -54.90051 | 1.000 | 0.0 | | 1.000 | 0.0 |
| T | 2a'1a" | -54.47494 | 0.998 | 0.4 | -54.88914 | 0.998 | 0.5 |
| | 4a'1a" | | 0.002 | | -54.46314 | 0.002 | |

Table S17: EOMDIP-CCSD and EOMDIP-CCSD(2) total energies in Hartree for dicationic states of water. The column "Weight" reports the square of the amplitude of the respective configuration divided by the square norm of $R_{ij}$. The energy of the neutral ground state is -76.39776/-76.39226 a.u. computed with CCSD and MP2, respectively.

| | | EOMDIP-CCSD | | | EOMDIP-CCSD(2) | | |
|---|---|---|---|---|---|---|---|
| Spin state | Configuration | Total energy | Weight | Partial width | Total energy | Weight | Partial width |
| S | $1b_2 1b_2$ | -74.85355 | 0.954 | 7.0 | -74.84079 | 0.953 | 10.2 |
| | $3a_1 3a_1$ | | 0.046 | | | 0.047 | |
| S | $3a_1 3a_1$ | -74.69050 | 0.941 | 5.3 | -74.68054 | 0.939 | 7.8 |
| | $1b_2 1b_2$ | | 0.039 | | | 0.040 | |
| | $1b_1 1b_1$ | | 0.020 | | | 0.021 | |
| S | $1b_1 1b_1$ | -74.42187 | 0.965 | 4.7 | -74.41466 | 0.964 | 6.3 |
| | $2a_1 2a_1$ | | 0.019 | | | 0.020 | |
| | $3a_1 3a_1$ | | 0.016 | | | 0.016 | |
| S | $2a_1 3a_1$ | -73.91846 | 1.000 | 5.7 | -73.90948 | 1.000 | 5.7 |
| S | $2a_1 2a_1$ | -73.24213 | 0.984 | 6.9 | -73.23637 | 0.984 | 6.3 |
| | $1b_1 1b_1$ | | 0.016 | | | 0.016 | |

| Spin | Transition | EOMDIP-CCSD Total | Weight | Partial | EOMDIP-CCSD(2) Total | Weight | Partial |
|---|---|---|---|---|---|---|---|
| T | $2a_13a_1$ | -74.14748 | 1.000 | 1.1 | -74.14001 | 1.000 | 1.1 |
| S | $1b_11b_2$ | -74.67715 | 1.000 | 6.1 | -74.66810 | 1.000 | 9.7 |
| T | $1b_11b_2$ | -74.74189 | 1.000 | 0.0 | -74.73310 | 1.000 | 0.0 |
| S | $3a_11b_1$ | -74.59839 | 1.000 | 7.3 | -74.59027 | 1.000 | 9.3 |
| S | $2a_11b_1$ | -73.73650 | 1.000 | 3.2 | -73.72979 | 1.000 | 3.9 |
| T | $3a_11b_1$ | -74.67509 | 1.000 | 0.1 | -74.66756 | 1.000 | 0.1 |
| T | $2a_11b_1$ | -74.00236 | 1.000 | 0.9 | -73.99643 | 1.000 | 0.9 |
| S | $3a_11b_2$ | -74.80208 | 1.000 | 7.3 | -74.79061 | 1.000 | 11.2 |
| S | $2a_11b_2$ | -73.96431 | 1.000 | 5.4 | -73.95472 | 1.000 | 5.0 |
| T | $3a_11b_2$ | -74.89105 | 1.000 | 0.1 | -74.88006 | 1.000 | 0.1 |
| T | $2a_11b_2$ | -74.21008 | 1.000 | 1.3 | -74.20143 | 1.000 | 1.1 |

Table S18: EOMDIP-CCSD and EOMDIP-CCSD(2) total energies in Hartree for dicationic states of silane. The column "Weight" reports the square of the amplitude of the respective configuration divided by the square norm of $R_{ij}$. All states that involve the 2a orbital were obtained by the extrapolation shown in Figs. S5 and S6. The energy of the neutral ground state is -291.79168/-291.76037 a.u. computed with CCSD and MP2, respectively.

| Spin state | Configuration | EOMDIP-CCSD Total energy | Weight | Partial width | EOMDIP-CCSD(2) Total energy | Weight | Partial width |
|---|---|---|---|---|---|---|---|
| S | $2b_12b_1$ | -290.57388 | 0.558 | 0.0 | -290.55389 | 0.511 | 0.0 |
| | $2b_22b_2$ | | 0.434 | | | 0.489 | |
| | $2b_32b_3$ | | 0.008 | | | 0.000 | |
| S | $2b_32b_3$ | -290.57388 | 0.657 | 0.0 | -290.55389 | 0.667 | 0.0 |
| | $2b_22b_2$ | | 0.240 | | | 0.172 | |
| | $2b_12b_1$ | | 0.103 | | | 0.162 | |
| S | $2b_12b_2$ | -290.50057 | 0.830 | 0.0 | -290.47928 | 0.823 | 0.0 |
| | $3a2b_3$ | | 0.170 | | | 0.177 | |
| S | $2b_12b_3$ | -290.50057 | 0.830 | 0.0 | -290.47928 | 0.823 | 0.0 |
| | $3a2b_2$ | | 0.170 | | | 0.177 | |
| S | $2b_22b_3$ | -290.50057 | 0.830 | 0.0 | -290.47928 | 0.823 | 0.0 |
| | $3a2b_1$ | | 0.170 | | | 0.177 | |
| S | $2b_22b_2$ | -290.39803 | 0.294 | 0.0 | -290.37348 | 0.292 | 0.0 |
| | $2b_32b_3$ | | 0.294 | | | 0.292 | |
| | $2b_12b_1$ | | 0.294 | | | 0.292 | |
| | 3a3a | | 0.117 | | | 0.123 | |

| | | EOMDIP-CCSD | | | EOMDIP-CCSD(2) | | |
|---|---|---|---|---|---|---|---|
| Spin state | Transition | Total energy | Weight | Partial width | Total energy | Weight | Partial width |
| S | $3a2b_1$ | -290.17045 | 0.816 | 0.0 | -290.14470 | 0.806 | 0.0 |
| | $2b_22b_3$ | | 0.184 | | | 0.195 | |
| S | $3a2b_2$ | -290.17045 | 0.816 | 0.0 | -290.14470 | 0.806 | 0.0 |
| | $2b_12b_3$ | | 0.184 | | | 0.195 | |
| S | $3a2b_3$ | -290.17045 | 0.816 | 0.0 | -290.14470 | 0.806 | 0.0 |
| | $2b_12b_2$ | | 0.184 | | | 0.195 | |
| S | 3a3a | -290.01533 | 0.862 | 0.0 | -289.99245 | 0.856 | 0.0 |
| | $2b_22b_2$ | | 0.046 | | | 0.048 | |
| | $2b_32b_3$ | | 0.046 | | | 0.048 | |
| | $2b_12b_1$ | | 0.046 | | | 0.048 | |
| S | $1b_12b_2$ | -286.98579 | 0.500 | 0.3 | -286.95375 | 0.500 | 0.3 |
| | $2b_11b_2$ | | 0.500 | | | 0.500 | |
| S | $2b_11b_3$ | -286.98579 | 0.500 | 0.3 | -286.95375 | 0.500 | 0.3 |
| | $1b_12b_3$ | | 0.500 | | | 0.500 | |
| S | $2b_21b_3$ | -286.98579 | 0.500 | 0.3 | -286.95375 | 0.500 | 0.3 |
| | $1b_22b_3$ | | 0.500 | | | 0.500 | |
| S | $1b_22b_3$ | -286.94955 | 0.499 | 0.3 | -286.90481 | 0.499 | 0.3 |
| | $2b_21b_3$ | | 0.499 | | | 0.499 | |
| | $1b_21b_3$ | | 0.001 | | | 0.001 | |
| S | $2b_11b_2$ | -286.94955 | 0.499 | 0.3 | -286.90481 | 0.499 | 0.3 |
| | $1b_12b_2$ | | 0.499 | | | 0.499 | |
| | $1b_11b_2$ | | 0.001 | | | 0.001 | |
| S | $2b_11b_3$ | -286.94955 | 0.499 | 0.3 | -286.90481 | 0.499 | 0.3 |
| | $1b_12b_3$ | | 0.499 | | | 0.499 | |
| | $1b_11b_3$ | | 0.001 | | | 0.001 | |
| S | $1b_22b_2$ | -286.94465 | 0.638 | 0.5 | -286.91526 | 0.625 | 0.5 |
| | $1b_32b_3$ | | 0.296 | | | 0.327 | |
| | $1b_12b_1$ | | 0.065 | | | 0.048 | |
| | $1b_21b_2$ | | 0.001 | | | 0.001 | |
| S | $1b_22b_2$ | -286.94465 | 0.638 | 0.5 | -286.91526 | 0.662 | 0.5 |
| | $1b_32b_3$ | | 0.296 | | | 0.211 | |
| | $1b_12b_1$ | | 0.065 | | | 0.126 | |
| | $1b_21b_2$ | | 0.001 | | | 0.001 | |
| S | $1b_32b_3$ | -286.92978 | 0.333 | 0.5 | -286.90011 | 0.332 | 0.5 |
| | $1b_12b_1$ | | 0.333 | | | 0.332 | |
| | $1b_22b_2$ | | 0.333 | | | 0.332 | |
| | 2a3a | | 0.001 | | | 0.001 | |

| | | EOMDIP-CCSD | | | EOMDIP-CCSD(2) | | |
|---|---|---|---|---|---|---|---|
| Spin state | Transition | Total energy | Weight | Partial width | Total energy | Weight | Partial width |
| S | $3a1b_1$ | -286.67097 | 0.998 | 0.4 | -286.63726 | 0.997 | 0.4 |
| | $2a2b_1$ | | 0.001 | | | 0.001 | |
| | $2b_21b_3$ | | 0.000 | | | 0.001 | |
| | $1b_22b_3$ | | 0.000 | | | 0.001 | |
| S | $3a1b_2$ | -286.67097 | 0.998 | 0.4 | -286.63726 | 0.997 | 0.4 |
| | $2a2b_2$ | | 0.001 | | | 0.001 | |
| | $2b_11b_3$ | | 0.000 | | | 0.001 | |
| | $1b_12b_3$ | | 0.000 | | | 0.001 | |
| S | $3a1b_3$ | -286.67097 | 0.998 | 0.4 | -286.63726 | 0.997 | 0.4 |
| | $2a2b_3$ | | 0.001 | | | 0.001 | |
| | $1b_12b_2$ | | 0.000 | | | 0.001 | |
| | $2b_11b_2$ | | 0.000 | | | 0.001 | |
| S | $2a2b_1$ | -285.29962 | 0.998 | 0.2 | -285.26726 | 0.998 | 0.2 |
| S | $2a2b_2$ | -285.29962 | 0.998 | 0.2 | -285.26726 | 0.998 | 0.2 |
| S | $2a2b_3$ | -285.29962 | 0.998 | 0.2 | -285.26726 | 0.998 | 0.2 |
| S | 2a3a | -285.00274 | 0.998 | 0.8 | -284.97138 | 0.998 | 0.7 |
| S | $1b_11b_2$ | -282.39659 | 0.999 | 10.8 | -282.35105 | 0.999 | 12.5 |
| | $1b_12b_2$ | | 0.001 | | | 0.000 | |
| | $2b_11b_2$ | | 0.001 | | | 0.000 | |
| S | $1b_11b_3$ | -282.39659 | 0.999 | 10.8 | -282.35105 | 0.999 | 12.5 |
| | $1b_12b_3$ | | 0.001 | | | 0.000 | |
| | $2b_11b_3$ | | 0.001 | | | 0.000 | |
| S | $1b_21b_3$ | -282.39659 | 0.999 | 10.8 | -282.35105 | 0.999 | 12.5 |
| | $2b_21b_3$ | | 0.001 | | | 0.000 | |
| | $1b_22b_3$ | | 0.001 | | | 0.000 | |
| S | $1b_31b_3$ | -282.39540 | 0.639 | 8.1 | -282.34784 | 0.655 | 9.3 |
| | $1b_21b_2$ | | 0.292 | | | 0.245 | |
| | $1b_11b_1$ | | 0.067 | | | 0.099 | |
| | $1b_32b_3$ | | 0.001 | | | 0.001 | |
| S | $1b_31b_3$ | -282.39540 | 0.574 | 8.1 | -282.34784 | 0.655 | 9.3 |
| | $1b_11b_1$ | | 0.410 | | | 0.245 | |
| | $1b_21b_2$ | | 0.014 | | | 0.099 | |
| | $1b_32b_3$ | | 0.001 | | | 0.001 | |
| | $1b_12b_1$ | | 0.001 | | | 0.000 | |
| S | $1b_31b_3$ | -282.17591 | 0.323 | 8.0 | -282.13138 | 0.323 | 9.2 |
| | $1b_21b_2$ | | 0.323 | | | 0.323 | |
| | $1b_11b_1$ | | 0.323 | | | 0.323 | |
| | 2a2a | | 0.028 | | | 0.028 | |

| | | EOMDIP-CCSD | | | EOMDIP-CCSD(2) | | |
|---|---|---|---|---|---|---|---|
| Spin state | Transition | Total energy | Weight | Partial width | Total energy | Weight | Partial width |
| S | $2a1b_1$ | -280.46165 | 0.999 | 7.8 | -280.41387 | 0.999 | 8.3 |
| S | $2a1b_2$ | -280.46165 | 0.999 | 7.8 | -280.41387 | 0.999 | 8.3 |
| S | $2a1b_3$ | -280.46165 | 0.999 | 7.8 | -280.41387 | 0.999 | 8.3 |
| S | 2a2a | -279.02472 | 0.974 | 5.7 | -278.97842 | 0.973 | 5.1 |
| | $1b_11b_1$ | | 0.009 | | | 0.009 | |
| | $1b_21b_2$ | | 0.009 | | | 0.009 | |
| | $1b_31b_3$ | | 0.009 | | | 0.009 | |
| T | $2b_12b_2$ | -290.57814 | 1.000 | 0.0 | -290.55804 | 1.000 | 0.0 |
| T | $2b_12b_3$ | -290.57814 | 1.000 | 0.0 | -290.55804 | 1.000 | 0.0 |
| T | $2b_22b_3$ | -290.57814 | 1.000 | 0.0 | -290.55804 | 1.000 | 0.0 |
| T | $3a2b_1$ | -290.35645 | 1.000 | 0.0 | -290.33608 | 1.000 | 0.0 |
| T | $3a2b_2$ | -290.35645 | 1.000 | 0.0 | -290.33608 | 1.000 | 0.0 |
| T | $3a2b_3$ | -290.35645 | 1.000 | 0.0 | -290.33608 | 1.000 | 0.0 |
| T | $1b_12b_1$ | -286.97729 | 0.558 | 0.0 | -286.94507 | 0.560 | 0.0 |
| | $1b_22b_2$ | | 0.434 | | | 0.431 | |
| | $1b_32b_3$ | | 0.008 | | | 0.008 | |
| T | $1b_32b_3$ | -286.97729 | 0.631 | 0.0 | -286.94507 | 0.658 | 0.0 |
| | $1b_22b_2$ | | 0.315 | | | 0.235 | |
| | $1b_12b_1$ | | 0.054 | | | 0.106 | |
| T | $2b_11b_2$ | -286.97268 | 0.500 | 0.0 | -286.94055 | 0.500 | 0.0 |
| | $1b_12b_2$ | | 0.500 | | | 0.500 | |
| T | $2b_11b_3$ | -286.97268 | 0.500 | 0.0 | -286.94055 | 0.500 | 0.0 |
| | $1b_12b_3$ | | 0.500 | | | 0.500 | |
| T | $2b_21b_3$ | -286.97268 | 0.500 | 0.0 | -286.94055 | 0.500 | 0.0 |
| | $1b_22b_3$ | | 0.500 | | | 0.500 | |
| T | $2b_21b_3$ | -286.96704 | 0.500 | 0.0 | -286.92773 | 0.500 | 0.0 |
| | $1b_22b_3$ | | 0.500 | | | 0.500 | |
| | $1b_21b_3$ | | 0.001 | | | 0.001 | |
| T | $1b_12b_3$ | -286.96704 | 0.500 | 0.0 | -286.92773 | 0.500 | 0.0 |
| | $2b_11b_3$ | | 0.500 | | | 0.500 | |
| | $1b_11b_3$ | | 0.001 | | | 0.001 | |
| T | $2b_11b_2$ | -286.96704 | 0.500 | 0.0 | -286.92773 | 0.500 | 0.0 |
| | $1b_12b_2$ | | 0.500 | | | 0.500 | |
| | $1b_11b_2$ | | 0.001 | | | 0.001 | |
| T | $1b_32b_3$ | -286.96239 | 0.333 | 0.0 | -286.93018 | 0.333 | 0.0 |
| | $1b_12b_1$ | | 0.333 | | | 0.333 | |
| | $1b_22b_2$ | | 0.333 | | | 0.333 | |
| | 2a3a | | 0.001 | | | 0.001 | |
| T | $3a1b_1$ | -286.69460 | 1.000 | 0.1 | -286.65671 | 0.999 | 0.1 |

| Spin state | Transition | EOMDIP-CCSD Total energy | EOMDIP-CCSD Weight | EOMDIP-CCSD Partial width | EOMDIP-CCSD(2) Total energy | EOMDIP-CCSD(2) Weight | EOMDIP-CCSD(2) Partial width |
|---|---|---|---|---|---|---|---|
| T | $3a1b_2$ | -286.69460 | 1.000 | 0.1 | -286.65671 | 0.999 | 0.1 |
| T | $3a1b_3$ | -286.69460 | 1.000 | 0.1 | -286.65671 | 0.999 | 0.1 |
| T | $2a2b_1$ | -285.30503 | 0.999 | 0.0 | -285.27255 | 0.999 | 0.0 |
| T | $2a2b_2$ | -285.30503 | 0.999 | 0.0 | -285.27255 | 0.999 | 0.0 |
| T | $2a2b_3$ | -285.30503 | 0.999 | 0.0 | -285.27255 | 0.999 | 0.0 |
| T | 2a3a | -285.02899 | 0.999 | 0.0 | -284.99702 | 0.999 | 0.0 |
| T | $1b_11b_3$ | -282.59555 | 0.999 | 0.0 | -282.55007 | 0.999 | 0.0 |
| T | $1b_11b_2$ | -282.59555 | 0.999 | 0.0 | -282.55007 | 0.999 | 0.0 |
| T | $1b_21b_3$ | -282.59555 | 0.999 | 0.0 | -282.55007 | 0.999 | 0.0 |
| T | $2a1b_1$ | -281.05384 | 0.999 | 1.5 | -281.00736 | 0.999 | 1.6 |
| T | $2a1b_2$ | -281.05384 | 0.999 | 1.5 | -281.00736 | 0.999 | 1.6 |
| T | $2a1b_3$ | -281.05384 | 0.999 | 1.5 | -281.00736 | 0.999 | 1.6 |

Table S19: EOMDIP-CCSD and EOMDIP-CCSD(2) total energies in Hartree for dicationic states of phosphine. The column "Weight" reports the square of the amplitude of the respective configuration divided by the square norm of $R_{ij}$. All states that involve the 2a' orbital were obtained by the extrapolation shown in Figs. S3 and S4. The energy of the neutral ground state is -343.05079/-343.02280 a.u. computed with CCSD and MP2, respectively.

| Spin state | Configuration | EOMDIP-CCSD Total energy | EOMDIP-CCSD Weight | EOMDIP-CCSD Partial width | EOMDIP-CCSD(2) Total energy | EOMDIP-CCSD(2) Weight | EOMDIP-CCSD(2) Partial width |
|---|---|---|---|---|---|---|---|
| S | 1a"1a" | -331.28485 | 0.484 | 8.7 | -331.23337 | 0.492 | 9.2 |
| | 3a'3a' | | 0.483 | | | 0.492 | |
| | 3a'4a' | | 0.032 | | | 0.015 | |
| | 1a"2a" | | 0.001 | | | 0.001 | |
| | 3a'6a' | | 0.001 | | | 0.001 | |
| S | 1a"1a" | -331.03945 | 0.328 | 8.5 | -330.98761 | 0.328 | 9.1 |
| | 3a'3a' | | 0.328 | | | 0.328 | |
| | 4a'4a' | | 0.314 | | | 0.314 | |
| | 2a'2a' | | 0.027 | | | 0.027 | |
| | 2a'5a' | | 0.001 | | | 0.001 | |
| | 1a"2a" | | 0.001 | | | 0.001 | |
| | 3a'6a' | | 0.001 | | | 0.001 | |
| | 4a'7a' | | 0.001 | | | 0.001 | |

| | | EOMDIP-CCSD | | | EOMDIP-CCSD(2) | | |
|---|---|---|---|---|---|---|---|
| Spin state | Transition | Total energy | Weight | Partial width | Total energy | Weight | Partial width |
| S | 1a”2a” | -337.00007 | 0.488 | 0.6 | -336.96617 | 0.488 | 0.6 |
| | 3a’6a’ | | 0.488 | | | 0.488 | |
| | 4a’7a’ | | 0.021 | | | 0.022 | |
| | 2a’5a’ | | 0.001 | | | 0.001 | |
| S | 2a’1a” | -329.10974 | 0.999 | 8.4 | -329.06201 | 0.999 | 8.7 |
| S | 2a’2a’ | -327.49306 | 0.974 | 5.8 | -327.44658 | 0.974 | 6.2 |
| | 4a’4a’ | | 0.008 | | | 0.008 | |
| S | 2a’2a” | -335.17422 | 0.998 | 0.3 | -335.14588 | 0.998 | 0.3 |
| S | 2a’3a’ | -329.10974 | 0.999 | 8.4 | -329.06201 | 0.999 | 8.7 |
| S | 2a’4a’ | -329.10887 | 0.999 | 8.4 | -329.06129 | 0.999 | 8.7 |
| S | 2a’5a’ | -334.76199 | 0.981 | 0.9 | -334.73439 | 0.981 | 1.1 |
| S | 2a’6a’ | -335.17422 | 0.998 | 0.3 | -335.14588 | 0.998 | 0.3 |
| S | 2a’7a’ | -335.24292 | 0.981 | 0.5 | -335.21430 | 0.981 | 0.6 |
| S | 2a”2a” | -341.67763 | 0.458 | 0.0 | -341.65616 | 0.456 | 0.0 |
| | 6a’6a’ | | 0.458 | | | 0.456 | |
| | 5a’6a’ | | 0.058 | | | 0.062 | |
| | 6a’7a’ | | 0.025 | | | 0.025 | |
| S | 3a’1a” | -331.28485 | 0.967 | 11.3 | -331.23337 | 0.984 | 11.5 |
| | 4a’1a” | | 0.032 | | | 0.015 | |
| | 3a’2a” | | 0.001 | | | 0.001 | |
| | 6a’1a” | | 0.001 | | | 0.001 | |
| S | 3a’2a” | -337.02182 | 0.497 | 0.4 | -336.98527 | 0.500 | 0.4 |
| | 6a’1a” | | 0.497 | | | 0.499 | |
| | 4a’2a” | | 0.006 | | | 0.000 | |
| | 3a’1a” | | 0.001 | | | 0.001 | |
| S | 3a’2a” | -337.01577 | 0.499 | 0.4 | -337.10146 | 0.000 | 0.5 |
| | 6a’1a” | | 0.499 | | | 0.000 | |
| | 3a’1a” | | 0.001 | | | 0.000 | |
| | 4a’2a” | | 0.000 | | | 0.076 | |
| | 7a’1a” | | 0.000 | | | 0.915 | |
| | 5a’1a” | | 0.000 | | | 0.009 | |
| S | 3a’4a’ | -331.28744 | 0.967 | 11.3 | -331.23569 | 0.964 | 11.6 |
| | 1a”1a” | | 0.016 | | | 0.018 | |
| | 3a’3a’ | | 0.016 | | | 0.018 | |
| | 3a’7a’ | | 0.001 | | | 0.001 | |
| | 4a’6a’ | | 0.001 | | | 0.001 | |
| S | 3a’5a’ | -336.66409 | 0.992 | 0.5 | -336.63080 | 0.992 | 0.5 |
| | 3a’7a’ | | 0.006 | | | 0.006 | |
| | 2a’6a’ | | 0.002 | | | 0.002 | |

| | | EOMDIP-CCSD | | | EOMDIP-CCSD(2) | | |
|---|---|---|---|---|---|---|---|
| Spin state | Transition | Total energy | Weight | Partial width | Total energy | Weight | Partial width |
| S | 3a'6a' | -337.02182 | 0.496 | 0.6 | -336.98527 | 0.499 | 0.6 |
| | 1a"2a" | | 0.496 | | | 0.499 | |
| | 4a'6a' | | 0.006 | | | 0.000 | |
| S | 3a'6a' | -337.01577 | 0.500 | 0.6 | -337.10146 | 0.000 | 0.5 |
| | 1a"2a" | | 0.499 | | | 0.000 | |
| | 4a'6a' | | 0.000 | | | 0.076 | |
| | 3a'7a' | | 0.000 | | | 0.915 | |
| | 3a'5a' | | 0.000 | | | 0.009 | |
| S | 4a'1a" | -331.28744 | 0.967 | 11.4 | -331.23569 | 0.964 | 11.6 |
| | 3a'1a" | | 0.031 | | | 0.035 | |
| | 7a'1a" | | 0.001 | | | 0.001 | |
| | 4a'2a" | | 0.001 | | | 0.001 | |
| S | 4a'2a" | -337.03737 | 0.923 | 0.4 | -337.00423 | 0.922 | 0.4 |
| | 7a'1a" | | 0.075 | | | 0.075 | |
| | 4a'1a" | | 0.001 | | | 0.001 | |
| | 6a'1a" | | 0.000 | | | 0.001 | |
| | 3a'2a" | | 0.000 | | | 0.001 | |
| S | 4a'4a' | -331.28820 | 0.677 | 8.6 | -331.23669 | 0.674 | 9.2 |
| | 3a'3a' | | 0.161 | | | 0.162 | |
| | 1a"1a" | | 0.161 | | | 0.162 | |
| | 4a'7a' | | 0.001 | | | 0.001 | |
| S | 4a'5a' | -336.66702 | 0.994 | 0.5 | -336.63431 | 0.994 | 0.5 |
| | 4a'7a' | | 0.003 | | | 0.003 | |
| | 2a'7a' | | 0.002 | | | 0.002 | |
| S | 4a'6a' | -337.03737 | 0.923 | 0.4 | -337.00423 | 0.922 | 0.4 |
| | 3a'7a' | | 0.075 | | | 0.075 | |
| | 3a'4a' | | 0.001 | | | 0.001 | |
| | 3a'6a' | | 0.000 | | | 0.001 | |
| | 1a"2a" | | 0.000 | | | 0.001 | |
| S | 4a'7a' | -337.09423 | 0.972 | 0.8 | -337.05916 | 0.968 | 0.9 |
| | 3a'6a' | | 0.010 | | | 0.012 | |
| | 1a"2a" | | 0.010 | | | 0.012 | |
| | 4a'5a' | | 0.006 | | | 0.007 | |
| | 4a'4a' | | 0.001 | | | 0.001 | |
| S | 5a'1a" | -336.66409 | 0.992 | 0.5 | -336.63080 | 0.992 | 0.5 |
| | 7a'1a" | | 0.006 | | | 0.006 | |
| | 2a'2a" | | 0.002 | | | 0.002 | |

| | | EOMDIP-CCSD | | | EOMDIP-CCSD(2) | | |
|---|---|---|---|---|---|---|---|
| Spin state | Transition | Total energy | Weight | Partial width | Total energy | Weight | Partial width |
| S | 5a'2a" | -341.31962 | 0.901 | 0.0 | -341.29905 | 0.887 | 0.0 |
| | 6a'2a" | | 0.073 | | | 0.083 | |
| | 7a'2a" | | 0.026 | | | 0.030 | |
| S | 5a'5a' | -341.06211 | 0.911 | 0.0 | -341.04117 | 0.904 | 0.1 |
| | 5a'7a' | | 0.030 | | | 0.033 | |
| | 6a'6a' | | 0.028 | | | 0.030 | |
| | 2a"2a" | | 0.028 | | | 0.030 | |
| | 7a'7a' | | 0.003 | | | 0.003 | |
| S | 5a'6a' | -341.31962 | 0.901 | 0.0 | -341.29906 | 0.887 | 0.0 |
| | 6a'6a' | | 0.036 | | | 0.041 | |
| | 2a"2a" | | 0.036 | | | 0.041 | |
| | 6a'7a' | | 0.026 | | | 0.030 | |
| S | 5a'7a' | -341.46451 | 0.949 | 0.0 | -341.44264 | 0.936 | 0.0 |
| | 6a'6a' | | 0.018 | | | 0.023 | |
| | 2a"2a" | | 0.018 | | | 0.023 | |
| | 5a'5a' | | 0.011 | | | 0.012 | |
| | 7a'7a' | | 0.005 | | | 0.005 | |
| S | 6a'1a" | -337.06576 | 0.500 | 0.4 | -337.03151 | 0.500 | 0.4 |
| | 3a'2a" | | 0.500 | | | 0.500 | |
| S | 6a'2a" | -341.67764 | 0.917 | 0.0 | -341.65617 | 0.913 | 0.0 |
| | 5a'2a" | | 0.058 | | | 0.062 | |
| | 7a'2a" | | 0.025 | | | 0.025 | |
| S | 6a'6a' | -341.60335 | 0.452 | 0.0 | -341.57933 | 0.449 | 0.0 |
| | 2a"2a" | | 0.452 | | | 0.449 | |
| | 5a'5a' | | 0.046 | | | 0.047 | |
| | 5a'7a' | | 0.034 | | | 0.037 | |
| | 7a'7a' | | 0.017 | | | 0.018 | |
| S | 6a'7a' | -341.81842 | 0.966 | 0.0 | -341.79843 | 0.964 | 0.0 |
| | 6a'6a' | | 0.015 | | | 0.017 | |
| | 2a"2a" | | 0.015 | | | 0.017 | |
| | 5a'6a' | | 0.003 | | | 0.003 | |
| S | 7a'2a" | -341.81843 | 0.966 | 0.0 | -341.79843 | 0.964 | 0.0 |
| | 6a'2a" | | 0.031 | | | 0.033 | |
| | 5a'2a" | | 0.003 | | | 0.003 | |
| S | 7a'7a' | -341.89757 | 0.968 | 0.0 | -341.87399 | 0.965 | 0.0 |
| | 5a'7a' | | 0.016 | | | 0.018 | |
| | 6a'6a' | | 0.007 | | | 0.007 | |
| | 2a"2a" | | 0.007 | | | 0.007 | |
| | 5a'5a' | | 0.003 | | | 0.003 | |

| | | EOMDIP-CCSD | | | EOMDIP-CCSD(2) | | |
|---|---|---|---|---|---|---|---|
| Spin state | Transition | Total energy | Weight | Partial width | Total energy | Weight | Partial width |
| T | 1a”2a” | -337.04403 | 0.498 | 0.0 | -337.00974 | 0.498 | 0.0 |
| | 3a’6a’ | | 0.498 | | | 0.498 | |
| | 4a’7a’ | | 0.003 | | | 0.004 | |
| T | 2a’1a” | -329.76786 | 0.999 | 1.6 | -329.72145 | 0.999 | 1.7 |
| T | 2a’2a” | -335.18141 | 0.999 | 0.1 | -335.15288 | 0.999 | 0.1 |
| T | 2a’3a’ | -329.76786 | 0.999 | 1.6 | -329.72145 | 0.999 | 1.7 |
| T | 2a’4a’ | -329.76734 | 0.999 | 1.6 | -329.72106 | 0.999 | 1.7 |
| T | 2a’5a’ | -334.79938 | 0.988 | 0.0 | -334.77106 | 0.988 | 0.0 |
| T | 2a’6a’ | -335.18141 | 0.999 | 0.1 | -335.15288 | 0.999 | 0.1 |
| T | 2a’7a’ | -335.25659 | 0.989 | 0.1 | -335.22780 | 0.989 | 0.1 |
| T | 3a’1a” | -331.51448 | 1.000 | 0.0 | -331.45396 | 1.000 | 0.0 |
| T | 3a’4a’ | -331.51291 | 1.000 | 0.0 | -331.45582 | 0.999 | 0.0 |
| T | 3a’5a’ | -336.69159 | 0.997 | 0.1 | -336.65830 | 0.997 | 0.1 |
| | 3a’7a’ | | 0.003 | | | 0.003 | |
| T | 3a’6a’ | -337.05410 | 0.454 | 0.0 | -337.02010 | 0.434 | 0.0 |
| | 1a”2a” | | 0.453 | | | 0.434 | |
| | 4a’6a’ | | 0.091 | | | 0.130 | |
| | 3a’7a’ | | 0.001 | | | 0.002 | |
| T | 3a’7a’ | -337.13966 | 0.985 | 0.0 | -337.10585 | 0.986 | 0.0 |
| | 4a’6a’ | | 0.010 | | | 0.009 | |
| | 3a’5a’ | | 0.005 | | | 0.005 | |
| T | 3a’1a” | -331.51030 | 0.999 | 0.0 | -331.45582 | 0.999 | 0.0 |
| T | 4a’2a” | -337.04785 | 0.901 | 0.0 | -337.01474 | 0.722 | 0.0 |
| | 3a’2a” | | 0.046 | | | 0.137 | |
| | 6a’1a” | | 0.046 | | | 0.137 | |
| | 7a’1a” | | 0.007 | | | 0.004 | |
| T | 4a’5a’ | -336.69445 | 0.996 | 0.1 | -336.66140 | 0.996 | 0.1 |
| | 4a’7a’ | | 0.003 | | | 0.003 | |
| T | 4a’6a’ | -337.04785 | 0.901 | 0.0 | -337.01474 | 0.723 | 0.0 |
| | 1a”2a” | | 0.046 | | | 0.136 | |
| | 3a’6a’ | | 0.046 | | | 0.136 | |
| | 3a’7a’ | | 0.007 | | | 0.004 | |
| T | 4a’7a’ | -337.14850 | 0.991 | 0.0 | -337.11432 | 0.990 | 0.0 |
| | 4a’5a’ | | 0.005 | | | 0.006 | |
| | 3a’6a’ | | 0.002 | | | 0.002 | |
| | 1a”2a” | | 0.002 | | | 0.002 | |
| T | 5a’1a” | -336.69159 | 0.997 | 0.1 | -336.65831 | 0.997 | 0.1 |
| | 7a’1a” | | 0.003 | | | 0.003 | |

| Spin state | Transition | EOMDIP-CCSD Total energy | Weight | Partial width | EOMDIP-CCSD(2) Total energy | Weight | Partial width |
|---|---|---|---|---|---|---|---|
| T | 5a'2a" | -341.45992 | 0.999 | 0.0 | -341.43985 | 0.999 | 0.0 |
| | 7a'2a" | | 0.001 | | | 0.001 | |
| T | 5a'6a' | -341.45992 | 0.999 | 0.0 | -341.43985 | 0.999 | 0.0 |
| | 6a'7a' | | 0.001 | | | 0.001 | |
| T | 5a'7a' | -341.58185 | 1.000 | 0.0 | -341.56180 | 1.000 | 0.0 |
| T | 6a'1a" | -337.05410 | 0.454 | 0.0 | -337.02010 | 0.434 | 0.0 |
| | 3a'2a" | | 0.453 | | | 0.434 | |
| | 4a'2a" | | 0.091 | | | 0.130 | |
| | 7a'1a" | | 0.001 | | | 0.002 | |
| T | 6a'1a" | -337.05410 | 0.454 | 0.0 | -337.02010 | 0.434 | 0.0 |
| | 3a'2a" | | 0.453 | | | 0.434 | |
| | 4a'2a" | | 0.091 | | | 0.130 | |
| | 7a'1a" | | 0.001 | | | 0.002 | |
| T | 6a'2a" | -341.73354 | 1.000 | 0.0 | -341.71365 | 1.000 | 0.0 |
| T | 6a'7a' | -341.85095 | 1.000 | 0.0 | -341.83141 | 1.000 | 0.0 |
| T | 7a'1a" | -337.13966 | 0.985 | 0.0 | -337.10586 | 0.986 | 0.0 |
| | 4a'2a" | | 0.010 | | | 0.009 | |
| | 5a'1a" | | 0.005 | | | 0.005 | |
| T | 7a'2a" | -341.85095 | 1.000 | 0.0 | -341.83141 | 1.000 | 0.0 |

Table S20: EOMDIP-CCSD and EOMDIP-CCSD(2) total energies in Hartree for dicationic states of hydrogen sulfide. The column "Weight" reports the square of the amplitude of the respective configuration divided by the square norm of $R_{ij}$. All states that involve the $2a_1$ orbital were obtained by the extrapolation shown in Figs. S1 and S2. The energy of the neutral ground state is -399.29963/-399.27754 a.u. computed with CCSD and MP2, respectively.

| Spin state | Configurations | EOMDIP-CCSD Total energy | Weight | Partial width | EOMDIP-CCSD(2) Total energy | Weight | Partial width |
|---|---|---|---|---|---|---|---|
| S | $2a_1 2a_1$ | -380.74178 | 0.992 | 11.7 | -380.70910 | 1.000 | 12.9 |
| S | $2a_1 1b_1$ | -382.53474 | 1.000 | 17.6 | -382.49810 | 1.000 | 18.0 |
| S | $2a_1 3a_1$ | -382.53527 | 1.000 | 17.6 | -382.49857 | 1.000 | 17.9 |
| S | $2a_1 1b_2$ | -382.53572 | 1.000 | 17.6 | -382.49886 | 1.000 | 17.9 |
| T | $2a_1 1b_1$ | -383.25703 | 1.000 | 3.2 | -383.22043 | 1.000 | 3.4 |
| T | $2a_1 3a_1$ | -383.25725 | 1.000 | 3.2 | -383.22061 | 1.000 | 3.4 |
| T | $2a_1 1b_2$ | -383.25752 | 1.000 | 3.2 | -383.22073 | 1.000 | 3.4 |

| | | EOMDIP-CCSD | | | EOMDIP-CCSD(2) | | |
|---|---|---|---|---|---|---|---|
| Spin state | Transition | Total energy | Weight | Partial width | Total energy | Weight | Partial width |
| S | $1b_21b_2$ | -384.65105 | 0.333 | 18.1 | -384.60505 | 0.576 | 18.4 |
| | $3a_13a_1$ | | 0.329 | | | 0.406 | |
| | $1b_11b_1$ | | 0.312 | | | 0.018 | |
| | $2a_12a_1$ | | 0.026 | | | 0.026 | |
| S | $3a_11b_2$ | -384.92245 | 1.000 | 24.6 | -384.87737 | 1.000 | 23.1 |
| S | $1b_21b_2$ | -384.92272 | 0.577 | 18.4 | -384.87906 | 0.661 | 18.2 |
| | $3a_13a_1$ | | 0.405 | | | 0.224 | |
| | $1b_11b_1$ | | 0.018 | | | 0.115 | |
| S | $1b_11b_2$ | -384.92618 | 1.000 | 24.3 | -384.87972 | 1.000 | 22.6 |
| S | $3a_11b_1$ | -384.92777 | 1.000 | 24.3 | -384.88091 | 1.000 | 22.7 |
| S | $1b_11b_1$ | -384.92812 | 0.640 | 18.2 | -384.88212 | 0.640 | 18.6 |
| | $3a_13a_1$ | | 0.312 | | | 0.312 | |
| | $1b_21b_2$ | | 0.048 | | | 0.048 | |
| T | $3a_11b_2$ | -385.16397 | 1.000 | 0.0 | -385.11593 | 1.000 | 0.0 |
| T | $1b_11b_2$ | -385.16579 | 1.000 | 0.0 | -385.12036 | 1.000 | 0.0 |
| T | $3a_11b_1$ | -385.16766 | 1.000 | 0.0 | -385.12169 | 1.000 | 0.0 |
| S | $2a_14a_1$ | -389.39167 | 1.000 | 2.1 | -389.36240 | 1.000 | 2.5 |
| T | $2a_14a_1$ | -389.44167 | 1.000 | 0.0 | -389.41162 | 1.000 | 0.0 |
| S | $2a_12b_2$ | -389.88555 | 1.000 | 0.8 | -389.85426 | 1.000 | 0.8 |
| T | $2a_12b_2$ | -389.89551 | 1.000 | 0.2 | -389.86397 | 1.000 | 0.1 |
| S | $2a_15a_1$ | -389.92156 | 1.000 | 1.2 | -389.88959 | 1.000 | 1.2 |
| T | $2a_15a_1$ | -389.93710 | 1.000 | 0.2 | -389.90493 | 1.000 | 0.2 |
| S | $2a_12b_1$ | -390.01347 | 1.000 | 1.2 | -389.98128 | 1.000 | 1.2 |
| T | $2a_12b_1$ | -390.02902 | 1.000 | 0.2 | -389.99662 | 1.000 | 0.2 |
| S | $4a_11b_2$ | -391.50805 | 1.000 | 1.2 | -391.47848 | 1.000 | 1.2 |
| S | $3a_14a_1$ | -391.50812 | 1.000 | 1.2 | -391.47973 | 1.000 | 1.2 |
| S | $4a_11b_1$ | -391.51614 | 1.000 | 1.2 | -391.48759 | 1.000 | 1.2 |
| T | $4a_11b_2$ | -391.53342 | 1.000 | 0.2 | -391.50714 | 1.000 | 0.2 |
| T | $3a_14a_1$ | -391.54028 | 1.000 | 0.2 | -391.51128 | 1.000 | 0.2 |
| T | $4a_11b_1$ | -391.54571 | 1.000 | 0.2 | -391.51756 | 1.000 | 0.2 |
| S | $1b_22b_2$ | -391.89365 | 0.927 | 1.5 | -391.84793 | 1.000 | 1.5 |
| | $3a_15a_1$ | | 0.073 | | | 0.000 | |
| S | $3a_12b_2$ | -391.92273 | 0.833 | 1.0 | -391.89389 | 0.833 | 0.9 |
| | $5a_11b_2$ | | 0.167 | | | 0.167 | |
| S | $2b_11b_2$ | -391.93410 | 0.951 | 1.0 | -391.90517 | 0.951 | 0.9 |
| | $1b_12b_2$ | | 0.049 | | | 0.049 | |
| T | $3a_12b_2$ | -391.94041 | 0.969 | 0.0 | -391.91035 | 0.971 | 0.0 |
| | $5a_11b_2$ | | 0.031 | | | 0.029 | |
| T | $1b_22b_2$ | -391.94593 | 1.000 | 0.0 | -391.91583 | 1.000 | 0.0 |

| | | EOMDIP-CCSD | | | EOMDIP-CCSD(2) | | |
|---|---|---|---|---|---|---|---|
| Spin state | Transition | Total energy | Weight | Partial width | Total energy | Weight | Partial width |
| T | $2b_1 1b_2$ | -391.94798 | 1.000 | 0.0 | -391.91869 | 1.000 | 0.0 |
| S | $3a_1 5a_1$ | -391.94873 | 0.933 | 1.8 | -391.91972 | 0.933 | 1.8 |
| | $1b_2 2b_2$ | | 0.067 | | | 0.067 | |
| S | $5a_1 1b_1$ | -391.98548 | 0.904 | 1.2 | -391.95246 | 0.890 | 1.1 |
| | $3a_1 2b_1$ | | 0.096 | | | 0.110 | |
| T | $5a_1 1b_2$ | -392.00506 | 1.000 | 0.0 | -391.97095 | 1.000 | 0.0 |
| S | $5a_1 1b_2$ | -392.00615 | 0.821 | 1.2 | -391.97678 | 0.821 | 1.1 |
| | $3a_1 2b_2$ | | 0.179 | | | 0.179 | |
| T | $5a_1 1b_1$ | -392.00696 | 1.000 | 0.0 | -391.97737 | 1.000 | 0.0 |
| T | $3a_1 5a_1$ | -392.01102 | 1.000 | 0.0 | -391.98094 | 1.000 | 0.0 |
| S | $1b_1 2b_1$ | -392.04610 | 1.000 | 2.4 | -392.01678 | 1.000 | 2.4 |
| S | $1b_1 2b_2$ | -392.10138 | 0.946 | 1.4 | -392.07229 | 0.946 | 1.3 |
| | $2b_1 1b_2$ | | 0.054 | | | 0.054 | |
| T | $1b_1 2b_2$ | -392.10779 | 1.000 | 0.0 | -392.07830 | 1.000 | 0.0 |
| S | $3a_1 2b_1$ | -392.11116 | 0.899 | 1.4 | -392.08106 | 0.899 | 1.3 |
| | $5a_1 1b_1$ | | 0.101 | | | 0.101 | |
| T | $3a_1 2b_1$ | -392.11196 | 1.000 | 0.0 | -392.08173 | 1.000 | 0.0 |
| T | $1b_1 2b_1$ | -392.12382 | 1.000 | 0.0 | -392.09324 | 1.000 | 0.0 |
| S | $4a_1 4a_1$ | -397.06871 | 0.869 | 0.1 | -397.05171 | 0.869 | 0.1 |
| | $4a_1 5a_1$ | | 0.101 | | | 0.101 | |
| | $2b_2 2b_2$ | | 0.030 | | | 0.030 | |
| S | $4a_1 2b_2$ | -397.29553 | 1.000 | 0.1 | -397.27866 | 1.000 | 0.1 |
| S | $4a_1 5a_1$ | -397.48515 | 0.974 | 0.1 | -397.46808 | 0.974 | 0.1 |
| T | $4a_1 2b_2$ | -397.51107 | 1.000 | 0.0 | -397.49452 | 1.000 | 0.0 |
| S | $4a_1 2b_1$ | -397.56269 | 1.000 | 0.1 | -397.54555 | 1.000 | 0.1 |
| T | $4a_1 5a_1$ | -397.59880 | 1.000 | 0.0 | -397.58162 | 1.000 | 0.0 |
| T | $4a_1 2b_1$ | -397.68791 | 1.000 | 0.0 | -397.67068 | 1.000 | 0.0 |
| S | $2b_2 2b_2$ | -397.70788 | 0.933 | 0.0 | -397.68774 | 0.933 | 0.0 |
| | $5a_1 5a_1$ | | 0.039 | | | 0.039 | |
| | $4a_1 4a_1$ | | 0.029 | | | 0.029 | |
| S | $5a_1 2b_2$ | -397.82839 | 1.000 | 0.0 | -397.81042 | 1.000 | 0.0 |
| T | $5a_1 2b_2$ | -397.88710 | 1.000 | 0.0 | -397.87040 | 1.000 | 0.0 |
| S | $5a_1 5a_1$ | -397.89703 | 0.957 | 0.0 | -397.87799 | 0.957 | 0.0 |
| | $2b_2 2b_2$ | | 0.043 | | | 0.043 | |
| S | $2b_1 2b_2$ | -397.96118 | 1.000 | 0.1 | -397.94289 | 1.000 | 0.0 |
| T | $2b_1 2b_2$ | -397.99345 | 1.000 | 0.0 | -397.97583 | 1.000 | 0.0 |
| S | $5a_1 2b_1$ | -398.02620 | 1.000 | 0.1 | -398.00627 | 1.000 | 0.1 |
| T | $5a_1 2b_1$ | -398.07858 | 1.000 | 0.0 | -398.06117 | 1.000 | 0.0 |
| S | $2b_1 2b_1$ | -398.11993 | 0.986 | 0.1 | -398.09971 | 0.985 | 0.1 |
